# Supplementary material for: How Much Should We Trust Instrumental Variable Estimates in Political Science? Practical Advice Based on Over 60 Replicated Studies
Source: arXiv:2303.11399 source file (2023-11-07)
Supplement: Supplementary file 1 [file appendixtable.tex]

%longtable to summarize all the papers in a single table.

%\begin{longtable}{| p{.20\textwidth} | p{.80\textwidth} |} 

\begin{landscape}\scriptsize
\subsection{\large Summary of Replicated Papers}
\label{sec:paperlist}

\begin{longtable}{L{2.8cm} L{2.8cm} L{1.8cm} L{1.8cm} L{1.8cm} L{8cm}}
\caption{Summary of Replicated Papers} 
\label{tab:paperlist}\\
\hline\hline
 \multicolumn{1}{c}{\bf Paper}   & \multicolumn{1}{c}{\bf Instrument} & \multicolumn{1}{c}{\bf Treatment} & \multicolumn{1}{c}{\bf Outcome} &\multicolumn{1}{c}{\bf IV Type}& \multicolumn{1}{c}{\bf Justification for IV Validity}  \\ \hline 
  \multicolumn{6}{c}{\textbf{APSR}}\\\hline

  \cite{gerber2010}  & Being sent mail & Aligning party identification with latent partisanship & Voting and party alignment scale & Experiment & NA \\ \hline 
  
  % \cite{gerber2011}   & Assigned TV and ratio advertisement & Actual TV and ratio advertisement & Voter preference & Experiment & NA \\ \hline
  
  \cite{meredith2013} &Governor’s home county&Democratic governor&Down-ballot Democratic candidates’ vote share&Theory (Other)& ``The validity of the instruments hinges on the assumption that, conditional on the control variables, coattail effects are the only channel through which the place of birth or residence of a party’s gubernatorial candidate affects the vote shares received by its down-ballot candidates."(p.745)\\ \hline
  
  \cite{blattman2014}  & Assignment to treatment blocks& Mass education campaign for dispute resolution & Serious land dispute & Experiment & NA \\ \hline

  \cite{laitin2016}   &Geographic distance from the origins of writing & Language choice & Human development index &Theory (Geography)& ``[T]he distance from these sites of invention should have no independent impact on socioeconomic development today, except through the channel of affecting the probability of possessing a writing tradition." (p. 470) \\ \hline

  \cite{ritter2016} &Rainfall&Mobilized dissent&Repression&Theory (Weather)& ``[R]ainfall is an exogenous predictor of dissent onset, meeting the key criteria for the instrumental analysis to allow for causal inference."(p.89)\\ \hline

  \cite{croke2016} &Access to the secondary education&Education attainment&Political participation&Rules \& policy changes (Change in exposure)& ``There are, however, good reasons to believe that the secondary education reform only affects participation through its effect on educational attainment."(p.592) \\ \hline

  \cite{dower2018}  &  Level of serfdom & Frequency of unrest & Peasant representation and unrest &Theory (History)& ``After conditioning on these covariates, we are left with that portion of serfdom largely determined by idiosyncratic variation in land grants to the nobility decades or centuries before the zemstvo reform of 1864." (p. 133) \\ \hline
  
  \cite{dower2018}  &  Religious polarization & Frequency of unrest & Peasant representation and unrest &Theory (History)& ``After conditioning on these covariates, we are left with that portion of serfdom largely determined by idiosyncratic variation in land grants to the nobility decades or centuries before the zemstvo reform of 1864." (p. 133) \\ \hline
  
  \cite{nellis2018}   & Narrow victory by secular parties in a district & The proportion of MNA seats in a district won by secularist candidates & Religious violence &Theory (Election)& ``Our identifying assumption is that the outcomes of such close elections are as good as randomly decided." (p. 50) \\ \hline

  \cite{kapoor2018}&Changes in entry costs. &Number of independent candidates & Voter turnout&Rules \& policy changes (Change in exposure)& ``It is worth reiterating that the deposit increases had nothing to do with historical differences in voter and candidate participation across reserved and open constituencies." (p. 681) \\ \hline

  \cite{colantone2018global}  & Imports from China to the United States $\times$ local industrial structure & Regional-level import shock from China & Leave support in Brexit &Econometrics (Interaction)& ``[The ]instrument is meant to capture the variation in Chinese imports, which is due to the exogenous changes in supply conditions in China, rather than to domestic factors in the United Kingdom that could be correlated with electoral outcomes." (p. 206) \\ \hline

  % \cite{dorsch2019}  & Regional share of democracies & Democratization events & Gini coefficient&Theory (Diffusion)& ``Intuitively, we expect that what happens in the regional countries is not related to the degree of inequality in the domestic country $i$, except through its influence on domestic political institutions." (p. 390) \\ \hline 

  \cite{hager2019ethnic}  & Distance to the nearest location where armored military vehicles were stolen & Ethnic riots (destruction) & Prosocial behavior &Theory (Other)&  ``[W]e present a falsification test which corroborates that the instrument is unrelated to prosocial behavior in a sample of 136 nearby villages, thus underlining the exclusion restriction." (p. 1037) \\ \hline

  \cite{baccini2021}  & Bartik instrument & Manufacturing Layoffs &Change of Democratic Vote Share&Econometrics (Interaction) &  ``Since layoffs are not randomly assigned, we develop an instrumental variables strategy using shift-share methodology (Bartik 1991) derived from national layoff shocks, weighted by initial county-level employment.''(p.550)  \\ \hline

  \cite{hager2022does}  & Number of corrupted Catholic priests & Number of secret police officers &Resistance &Theory (History) & ``In the early days of the
regime, the secret police’s ability to servile citizens
depended critically on the cooperation of the Catholic
Church...Importantly, the corruptibility of priests was
plausibly exogenous: priests were sent to municipalities
by the Catholic Church, often when another priest had
retired.'' (p.565)  \\ \hline

  \cite{kuipers2022representational}  & Statewide assignment mandate & Civil service reform &Descriptive representation on an unrestricted sample &Rules \& policy changes (Assignment) & ``First, we assume that state-level mandates are a strong instrument for city adoption; we verify the strength of the instrument in the main presentation of the results. The exclusion restriction, which is untestable, seems a reasonable assumption in our case."(p.9)   \\ \hline

    \\
  \multicolumn{6}{c}{\textbf{AJPS}}\\\hline
  
  \cite{kocher2011}    & Past insurgent control & Aerial bombing  & Changes in local control&Theory (Other)& ``Because instrumental variables require only conditional independence between instruments and the error term, we need only assume that there are no unobserved hamlet-specific variables that affected insurgent control in July, August, and December 1969, but not in September of that year as well." (p. 212)  \\ \hline

 \cite{vernby2013}    & Immigration Inflow 1940–1950; immigration Inflow 1960–1967 &  Share of noncitizens in the electorate&Municipal education and social spending &Theory (History)& ``Furthermore, it is unlikely that the initial locations of these refugees were affected by the level of local public services, suggesting that the instrument is also valid." (p. 25) \\ \hline

  \cite{tajima2013}   & Distance to health station & Distance to police posts (as a proxy for exposure to military intervention) & Incidence of communal violence &Theory (Geography) & ``According to a Health Department official, primary health stations must be located
in every subdistrict at their population centers, regardless
of the propensity for violence of those locations" (p. 112) \\ \hline

  \cite{delao2013}   & Random assignment to early coverage& Early coverage of Conditional Cash Transfer & Incumbent party's vote share & Experiment & NA \\ \hline

  \cite{mcclendon2014}   & Assignment to treatment & Reading social esteem promising email & Participation in LGBTQ events & Experiment & NA \\ \hline

% \cite{gerber2015}   & Assignment to treatment & Nonreturned mails & Voter turnout & Experiment & NA \\ \hline

\cite{barth2015}     & Adjusted bargaining coverage and effective number of union confederations & Wage inequality & Welfare support&Theory (Other)&  ``Yet conditional on union density and country fixed effects, we argue that certain properties of the bargaining system are likely to affect wages, but not union involvement in politics." (p. 574) \\ \hline

\cite{stokes2016}   &  Wind speed &Turbine location & Vote turnout &Theory (Climate)&  ``Wind speed is theoretically orthogonal to precinct boundaries but predicts the placement of wind turbine locations." (p. 965) \\ \hline

\cite{coppock2016} &Mailing showing 2005 Vote&Voting in November 2007 municipal elections&Voting in the 2008 presidential primary& Experiment & NA \\ \hline

\cite{trounstine2016}   & The number of waterways in a city combined with logged population & Racial segregation &Direct general expenditures &Theory (Geography) & ``I focus on waterways (including large streams and rivers), which vary in number across cities and are arguably exogenous to segregation and spending." (p. 717) \\ \hline

\cite{carnegie2017}    & Being a former colony of one of the Council members & Foreign aid & CIRI Human Empowerment index & Theory (History)&  ``In 1965, the EU stipulated that countries would hold the presidency for 6 months at a time [...] and would rotate alphabetically according to each member state’s name as spelled in its own language. " (p. 676) \\ \hline

\cite{zhu2017}    & Weighted geographic distance from economic centers & MNC activity & Corruption & Theory (Geography)&  ``This instrumental variable (IV) is rooted in the gravity models of international trade and FDI flows." (p. 90) \\ \hline 

\cite{rueda2017}    & The size of the polling station & Actual polling place size &Citizens' reports of electoral manipulation &Rules \& policy changes (Fuzzy RD) &  ``The institutional rule predicts sharp reductions in the size of the average polling station of a municipality every time the number of registered voters reaches a multiple of the maximum number of voters allowed to vote in a polling station." (p. 173) \\ \hline

\cite{lelkes2017}   & State-level ROW index&Number of providers & Affective polarization (partisan hostility) &Theory (Other)&  ``[A]n index of state regulation of right-of-way laws strongly predicts the number of providers in a county, which, as we discuss later, is a good proxy for broadband uptake." (p. 4). \\ \hline 

\cite{goldstein2017}    & Direct flight from city to Washington DC & Lobbying spending & Total earmarks or grants awarded &Theory (Other)&  ``The existence of a direct flight captures the convenience of travel to Washington, DC, from each city." (p. 865) \\ \hline

\cite{spenkuch2018}   & Individual princes’ decisions concerning whether to adopt Protestantism &Religion of voters living in the same areas more than three and a half centuries later & Nazi vote share &Theory (History)&  ``The historical record, however, suggests that princes’ decisions may plausibly satisfy this exogeneity assumption, especially after controlling for economic conditions at the end of the Weimar Republic as well as all factors known to have influenced rulers." (p. 27) \\ \hline 

% \cite{escriba-folch2018}   & Time trend for received remittances in high-income OECD countries and a country’s average distance from the coast. & Remittances & Protests &Theory (Geography)&  ``Remittances received in high-income OECD countries are unlikely to directly influence political change in remittance-receiving non-OECD countries except through their indirect effect on remittances sent to other countries." (p. 895) \\ \hline

\cite{colantone2018}   & Chinese imports to the United States $\times$regional industrial structure & Regional import shock from China & Economic nationalism&Econometrics (Interaction)&  ``This instrument is meant to capture the variation in Chinese imports due to exogenous changes in supply conditions in China, rather than to domestic factors that could be correlated with electoral outcomes." (p. 6) \\ \hline

\cite{hager2019}    & Mean elevation & Equitable inheritance customs & Female representation &Theory (Geography; History)&  ``Rivers are exogenous, but no longer should have a strong effect on inequality other than through the treatment." (p. 767) \\ \hline %circle back to this re: river NOTE FOR MAC

\cite{hager2019}    & Distance to rivers & Equitable inheritance customs & Female representation &Theory (Geography; History)&  ``Rivers are exogenous, but no longer should have a strong effect on inequality other than through the treatment." (p. 767) \\ \hline %circle back to this re: river NOTE FOR MAC

\cite{chong2019}   & Treatment assignment in get-out-to-vote campaigns& Actual proportion of households treated in the locality & Voted in 2013 presidential election & Experiment & NA \\ \hline

\cite{kim2019}    & Population threshold & Democratic institutions& Women political engagement & Rules \& policy changes (Fuzzy RD)&  ``[L]ocalities with a population greater than 1,500 must create a municipal council [...] whereas those with a population below that threshold were free to choose between the status quo direct democracy and representative democracy." (p. 6). \\ \hline 

\cite{sexton2019}    &Soldier fatalities & Health budget&Welfare outcome &Theory (Other)&  ``We substantiate [the exclusion restriction] below by ruling out the key alternative channel that local insecurity could affect citizens’ use of health services." (p. 359) \\ \hline

\cite{lopez2022policy} &Assignment to treatment&Town-hall meetings&Voting behavior& Experiment & NA \\ \hline

\cite{blair2022peacekeeping}    &Average fragmentation of all ongoing PKO mandates&Fragmentation of any given PKO mandate&Process performance &Theory (Other)& ``We view the first of these assumptions as mostly uncontroversial. As discussed above, most PKO mandates are only loosely tailored to conditions in their host countries. It is highly unlikely that the mandates of all other PKOs in Africa are tailored to the host country conditions of any given PKO. This should mitigate independence concerns.'' (p.11)  \\ \hline

\cite{hong2022strongman}&Geographic terrain elevation and slope& NVM subsidies&Park’s vote share in 2012 &Theory (Geography)& ``The logic behind this choice is as follows: each village’s performance in the NVM is evaluated based on their baseline conditions. Therefore, an unfavorable terrain before the movement likely indicates an initial lack of infrastructure in a poorer environment, and thus gives a village an advantageous benchmark from which to generate a notable and visible improvement within a short period compared to other villages.'' (p.11) \\ \hline

\cite{wood2022campaign}    &Random audit&Incumbent found to have campaign finance violations&Legislator retired &Experiment&  NA \\ \hline

\\
\multicolumn{6}{c}{\textbf{JOP}}\\\hline

% \cite{gerber2011persuasive}  & Rule used to select which households received the mailings& Share of voters receiving the mailings &Vote share &rules \& policy changes (Fuzzy RD)& ``To estimate (1) by instrumental variables, we impose the exclusion restriction that mail-eligible voters from census blocks where ${forcing}_b$ is just above zero have the same propensity to vote for a Democratic candidate as mail-eligible voters from census blocks where ${forcing}_b$ is just below zero."(p.148)\\ \hline 

\cite{gehlbach2012}   &Whether the first ruler in a nondemocratic episode is a military leader &Age of ruling party less leader years in office & Private investment/GDP&Theory&  ``[D]ictators who come to power with the backing of the military require less popular support to remain in power and are therefore less likely to promote private investment by allowing supporters to organize." (p. 628) \\ \hline

\cite{healy2013}    & Whether the younger sibling is a sister & The share of a respondent’s siblings who are female & 1973 gender-role attitude & Theory (Others -- Biology)& ``However, under Assumption 1, all siblings have an impact only through the overall gender makeup of the household." (p. 1027) \\ \hline

\cite{dube2015} &US military aid to countries outside of Latin America&US military aid to Colombia&The number of paramilitary attacks&Theory (Diffusion)& ``The instrument is valid since US funding to the rest of the world is determined by the broad geopolitical outlook of the American government, reflecting factors such as the party of the president or other major world events, and can thus be considered exogenous to the conflict in Colombia."(p.256) \\ \hline

\cite{flores-macias2013}   & Lagged values of country's energy production & Trade volume & Foreign policy convergence &Theory (Other)& ``The logic is that trade and trade salience in Africa and Latin America are significantly related to countries’ energy production, but there is no reason to believe that either of them is correlated with the error term in the equation predicting foreign policy convergence" (p. 365) \\ \hline

\cite{charron2013}    & Consolidation of clientelistic networks in regions where rulers have historically less constraints to their decisions & Clientelism & Quality of government &Theory (History)& ``[W]e also find that constraints are directly correlated with current regional institutional quality (yet in his analysis regional GDP and GDP growth are used), thus rendering it an imperfect instrument for clientelism"(p.576) \\ \hline

\cite{kriner2014}   & Number of days Congress is in session & Committee investigations & Presidential approval &Theory (Other)& ``[T]here is no theoretical reason drawn from existing literatures to expect the calendar to be independently correlated with presidential approval." (p. 525)  \\ \hline

\cite{lorentzen2014}    & Large firm dominance in 1999 & Large firm dominance in 2007 & Pollution information transparency index &Econometrics (Lagged treatment)& ``[The instrument was measured] well before transparency reforms were a major focus of discussion."  (p. 187) \\ \hline

\cite{dietrich2015}  & Constructed "internal" excluded instrument& Economic aid & Transitions to multipartyism &Econometrics (Lewbel instrument)& ``[We]show that the excluded instruments are generally uncorrelated with alternative channels through which they might influence the outcome variables." (p. 223) \\ \hline

\cite{feigenbaum2015}    & Chinese exports to other economies $\times$local exposure & Localized trade shocks in congressional districts & Trade score &Econometrics (Interaction)&  ``[We] use an instrument that depends [...] on Chinese import growth to other rich, Western economies" and "the lagged version is unaffected by Chinese trade shock." (p.1019) \\ \hline

\cite{alt2016}    & Assignment to receiving an aggregate unemployment forecast& Unemployment expectations & Vote intention & Experiment & NA \\ \hline

\cite{johns2016}    & Trade stake of the rest of the world& The number of other countries that became third parties & Becoming a third party &Theory (Other)&  ``[E]ach state’s participation decision is not directly affected by the trade stake of other countries. The trade stake of other countries matters only to the extent that it shapes a player’s belief about how other countries will behave." (p. 99) \\ \hline

\cite{acharya2016political}  & Measures of the environmental suitability for growing cotton & Slave proportion in 1860 & proportion Democrat &Theory (History)& ``We present results from this analysis showing that, outside the South, the relationship between cotton suitability and political attitudes is either very small or in the opposite direction as in the South." (p. 628) \\ \hline

% \cite{marshall2016}    & 1947 school reform & Years of schooling & Vote conservatives &Rules \& policy changes (Change in exposure)& ``selection into cohorts in Britain is implausible since parents could not have precisely predicted the 1947 reform more than a decade in advance", "since cohorts born either side of the cutoff were first eligible to vote in the 1955 election, there is no differential “first election” effect" and "pretreatment demographic, socioeconomic, and labor market characteristics are essentially continuous" (p. 386). \\ \hline 

\cite{schleiter2016}    & Prime Minister dissolution power& Opportunistic election calling& Vote share of Prime Minister's party &Theory (Other)& ``The instrument correlates directly with the treatment of interest—opportunistic election calling—without being linked to anticipated incumbent electoral performance." (p. 840) \\ \hline

\cite{henderson2016mediating} &Rain around Election day&Democratic vote margins&Incumbent roll call positioning&Theory (Weather)& ``Rain several days before an election may dampen the willingness to make plans, arrange transportation, and schedule time off work to go to the polls."(p.657)\\ \hline

\cite{henderson2016mediating} &Rain around Election weekend&Democratic vote margins&Incumbent roll call positioning&Theory (Weather)& ``Rain several days before an election may dampen the willingness to make plans, arrange transportation, and schedule time off work to go to the polls."(p.657)\\ \hline

% \cite{rozenas2016office} &Proximity-weighted economic shock&Economic crises&measure of office insecurity&Theory (Other)& ``The analysis assumes that, conditional on the covariates, country-level effects and time trends, electoral manipulation is not directly correlated with the instrument (independence) and the instrument affects electoral manipulation only through domestic economy (exclusion restriction)."(p.244) \\ \hline

\cite{charron2017}    & Proportion of Protestant residents in a region; aggregate literacy in 1880& More developed bureaucracy & Percent of single bidders &Theory (History)& ``[C]ross-country data show that, while the least corrupted countries in the world all have had near universal literacy for decades, other countries considered highly corrupt, [...] have, for the entire postwar era, also been some of the most highly literate places in the world." (p.97)\\ \hline

\cite{west2017}  & IEM (prediction market) price &Obama win & Policy efficacy &Theory (Other)& ``The identifying assumption is that there is no unobservable factor that simultaneously affects black (female) political efficacy and perceptions of the likelihood of an Obama (Clinton) victory." (p.352)\\ \hline

\cite{stewart2017}    & Log total border length and the total number of that state’s neighbors & Foreign territorial control & Civilian casualties &Theory (Geography)& ``[T]he longer a state’s borders or the greater its number of neighbors, the more accessible border regions in neighboring states will be to rebels, independent of the dynamics of their conflict with the government. Further, total border length or the number of bordering states is not likely to affect rebel targeting of civilians other than through their effects on the likelihood of rebel group’s controlling foreign territory." (p. 291) \\ \hline

\cite{lerman2017}   & Born 1946 or 1947& Public (p 1) versus only private (p 0) health insurance & Support ACA &Rules \& policy changes (Change in exposure)& ``We can confirm across a host of observable covariates that these two age groups are similar on almost every dimension, with the exception of insurance." (p. 631) \\ \hline

\cite{grossman2017}   & The number of distinct landmasses; length of medium and small streams; over-time variation in the number of regional governments & Government fragmentation & Public goods provision &Theory (Geography / diffusion)& ``Territorial structure of neighboring countries will affect the local discourse on institutional reforms and increase the likelihood that a country will adopt similar reforms" and "The other two instruments build on the fact that administrative and political boundaries are drawn around geographic landmarks." (p. 831) \\ \hline

\cite{cirone2018}   & Random assignment of budget incumbents to bureaux& Budget committee service & Legislator sponsorship on a budget bill & Theory (Other) & ``Conceptually, the competitiveness of the randomly assigned group acts similarly to a form of encouragement design." (p. 953) \\ \hline

\cite{bhavnani2018}  & Early-career job assignment to districts &Bureaucrats’ embeddedness & Proportion of villages with high schools &Theory (Other)& ``[T]he IAS posting orders that we obtained suggest that heuristics such alphabetical order and serial number—which are arbitrary and orthogonal to district and officer characteristics—are used to match officers to districts." (p. 78) \\ \hline

\cite{pianzola2019}   & Random assignment of the e-mail treatment & Smartvote use & Vote intention & Experiment & NA \\ \hline

\cite{arias2019large}   & Trade shock $\times$ UK bond yield & Government expenditures & Regular leader turnover  &Econometrics (Interaction)& ``The logic here is that when costs of external borrowing are high, a government experiencing a trade shock is more likely to cut expenditures because the option of borrowing to maintain or increase expenditures is too costly. This interaction term is the excluded instrument while the Trade Shock variable is included in both the first- and the second-stage estimates" (p. 1519) \\ \hline

\cite{ziaja2020} &Constructed instrument&Number of democracy donors&Democracy scores&Econometrics (Interaction)& ``[T]here is no reason to believe that the gender composition of a donor country’s parliament should affect democracy in a recipient country directly."(p.439)\\ \hline

\cite{schubiger2021state} &counterinsurgent mobilization &exposure to state violence&Location of a community inside or outside the emergency zone &Theory(Geography)& ``Destination choices were typically driven by economic and social factors (e.g., Degregori 1998, 151; Del Pino 1996, 164). Moreover, it is unlikely that local residents were able to anticipate the boundaries of the emergency zones and whether, when, and where they would change over time." (p.1389) \\ \hline

\cite{digiuseppe2022us} &Echelon corridor & US support & Fiscal capacity & Theory(Geography)& ``Like Aklin and Kern (2019), we ﬁnd that the echelon is plausibly exogenous to a state’s capacity, property rights, or risk of conﬂict. Instead, whether a state is located in the echelon corridor is a function of happenstance geography.''(p.777)\\ \hline

\cite{lei2022private} &Whether the city has more than 3 million residents & Subway approval & Mayor promotion & Rules \& policy changes (Fuzzy RD)& ``the city’s population exceeds 3 million people, and (4) more than 30,000 people per hour are expected to use a subway line''(p.463)\\ \hline

\cite{urpelainen2022electoral} &Time trend multiplied by the wind resource of the electoral district & Wind turbine capacity & Democratic vote & Econometrics(Interaction)& ``Validity of the average wind resource instrument hinges on two criteria: relevance and exclusion restriction...''(pp.1313-1314)\\ \hline

\cite{webster2022social} &Treatment assignment & Percentage of angry words that a respondent wrote in emotional recall prompts & Social polarization & Experiment&NA \\ \hline
\multicolumn{6}{p{19cm}}{\scriptsize {\it\textbf{Note:}} Justifications are omitted in the case of randomized controlled trials.}

\end{longtable}
\end{landscape}
