# Supplementary material for: How Much Should We Trust Instrumental Variable Estimates in Political Science? Practical Advice Based on Over 60 Replicated Studies
Source: arXiv:2303.11399 source file (2023-11-07)
Supplement: Supplementary file 2 [file supp.pdf]

## A. Supplementary Materials – Appendix A

### Table of Contents

#### A.1. Additional Replication Results

##### A.1.1. Replication Sample

##### A.1.2. Instruments based on Climate/Weather/Geography/History

##### A.1.3. Comparison of Multiple $F$ Statistics

#### A.2. Monte Carlo Evidence

##### A.2.1. Comparing $F$ Tests for Detecting Weak Instruments

##### A.2.2. Explaining the 2SLS-OLS Discrepancy

#### A.3. Evaluating IV Validity

##### A.3.1 The ZFS Test and Modified Inference

##### A.3.2. Simulation Evidence

##### A.3.3. A Case Study

#### A.4. Summary of Replicated Papers

## A.1. Additional Information on the Replication Sample

### A.1.1. Replication Sample

Figure A1 plots the histograms of effective  $F$  statistics using experiment-generated IVs (dark gray) and non-experimental IVs (light gray). The median effective  $F$  for experimental and observational designs are 67.7 and 53.5, respectively.

FIGURE A1. HISTOGRAM OF EFFECTIVE  $F$  STATISTIC

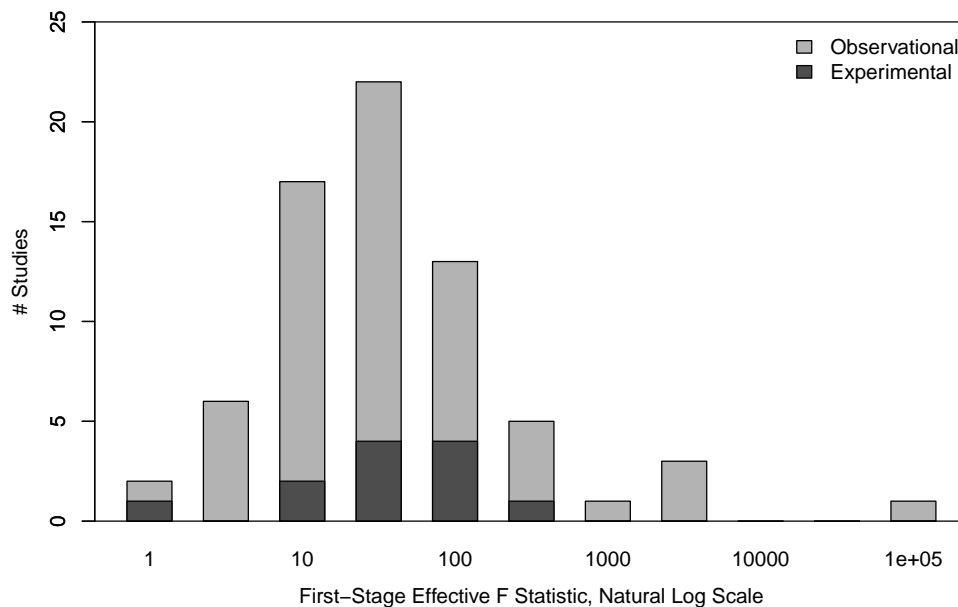

### A.1.2. Instruments based on Climate/Weather/Geography/History

Based on a reviewer's suggestion, we highlighted studies in Figure 4 that use “geography/climate/weather”, “history”, and “treatment diffusion” as IVs. We show that the inverse relationship between the first-stage correlation coefficient and the 2SLS-OLS ratio is consistent with other observational studies in our dataset.

FIGURE A2. INSTRUMENTS BASED ON CLIMATE/WEATHER/GEOGRAPHY/HISTORY

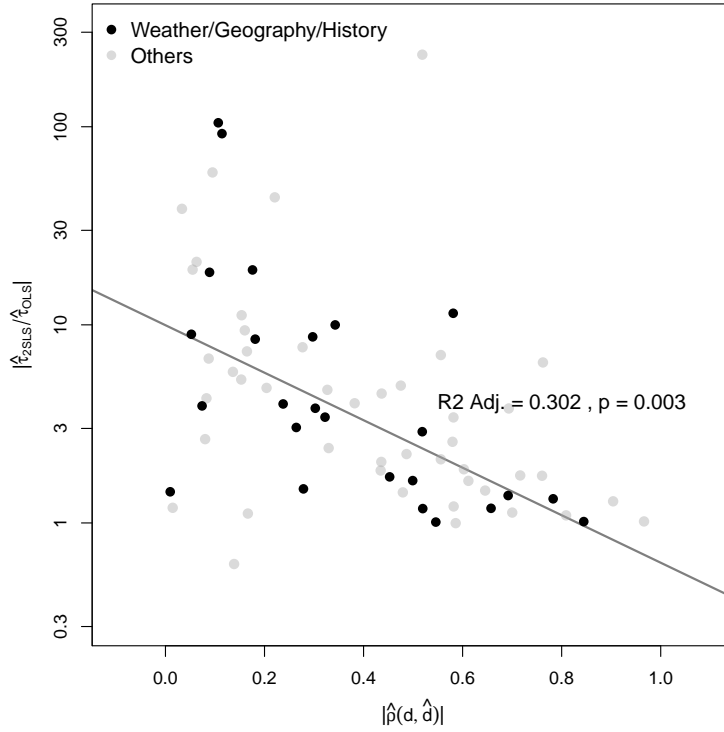

### A.1.3. Comparison of Multiple $F$ Statistics

Figure A3 compares the reported and replicated first-stage partial  $F$  statistics (for studies that have reported the  $F$  statistics). The replicated  $F$  statistics are based on the authors' chosen model specifications and variance estimators in 2SLS estimation. The discrepancy arises from the fact that some authors report the first-stage  $F$  statistic based on a different variance estimator than the one used in the 2SLS estimation. In the paper, we use the replicated ones to maintain consistency.

FIGURE A3. REPORTED VS. REPLICATED  $F$  STATISTICS

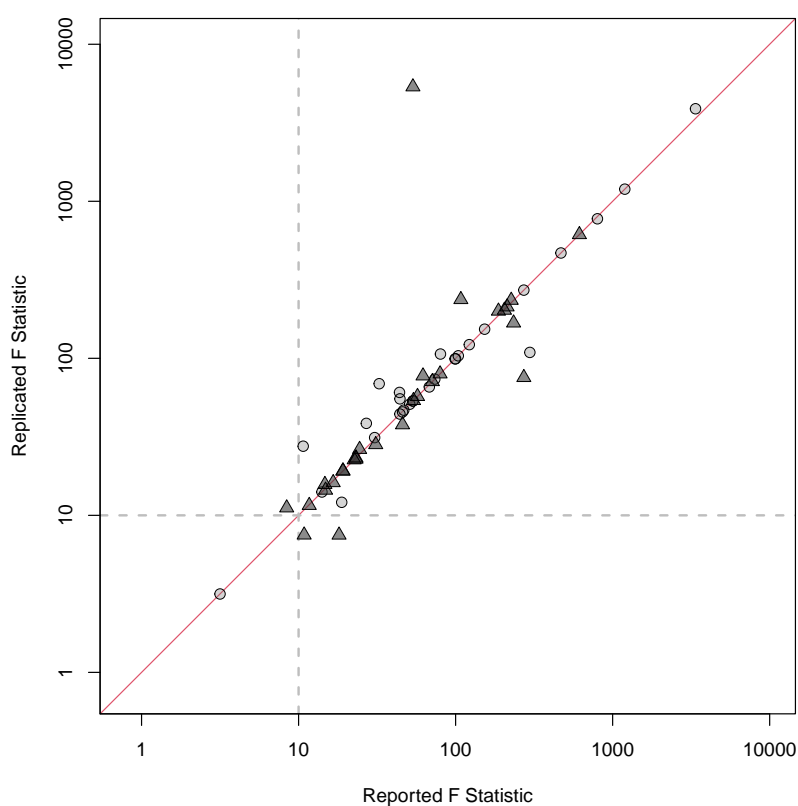

**Note:** Circles represent applications without a clustering structure and triangles represent applications with a clustering structure. Studies that do not report  $F$  statistics are not shown.

In Figure A4, we compare the traditional  $F$  statistics (based on classic analytic SEs), the Huber White robust  $F$  statistics, the effective  $F$  statistics (robust or cluster-bootstrap SEs) and (cluster-)bootstrapped  $F$  statistics. It shows that (cluster-)bootstrapped  $F$  statistics are usually the most conservative (smallest).

FIGURE A4. COMPARISON OF DIFFERENT  $F$  STATISTICS

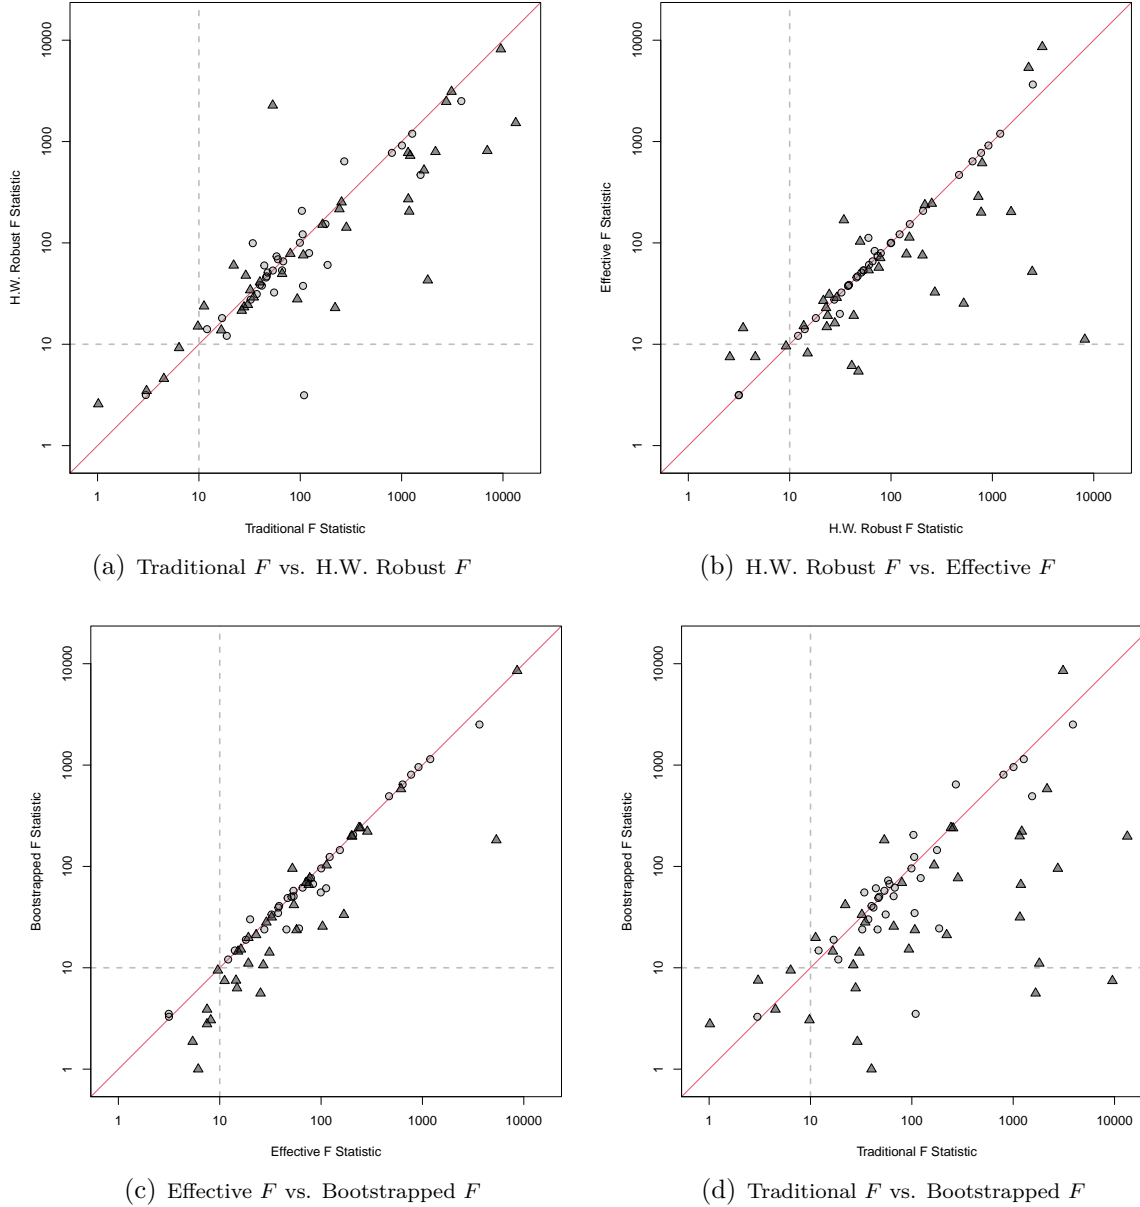

**Note:** Circles represent applications without a clustering structure and triangles represent applications with a clustering structure.

## A.2. Monte Carlo Evidence

### A.2.1. Comparing $F$ Tests for Detecting Weak Instruments

We conduct a simulation study with a clustered DGP in order to evaluate the relative performance of analytic and bootstrap  $F$  tests to detect weak instruments. We simulate data from the following DGP

$$\begin{aligned} \text{clustered instrument and error components } \nu_j, \eta_j &\sim \mathcal{N}(0, 0.5) \\ \text{instrument } z_i &\sim \mathcal{N}(0, 1) + \nu_j \\ \text{error } \varepsilon_i &\sim \mathcal{N}(0, 1) + \eta_j \\ \text{endogenous variable } x_i &= \pi z_i + \varepsilon_i \end{aligned}$$

with errors and instrument components drawn from  $J$  clusters. This DGP ensures that the data has a dependent structure within each cluster  $j$ . We then evaluate the strength of the instrument analytically by computing the t-statistic for  $H_0 : \pi = 0$ , or by using the corresponding bootstrap statistic  $\frac{\pi^2}{\hat{\sigma}^2}$  where  $\hat{\sigma}^2$  is the bootstrap estimate of the variance of  $\pi$ . We evaluate the analytic and bootstrap  $F$  statistics for various values of  $\pi$  and  $J$  for 100 replications of the above DGP in Figure (A5).

As seen in panel A, when robust analytic standard errors ignore the clustered structure, they vastly over-estimate the strength of the instrument relative to the cluster-bootstrap, with both “few” (10) and “many” (50) clusters and with “strong” ( $\pi = 0.5$ ) and “weak” ( $\pi = 0.001$ ) instruments. With appropriate clustered analytic SEs, however, the  $F$  statistic is typically comparable to the bootstrap based equivalent (panel B), although the bootstrap  $F$  is marginally more conservative with a small number of clusters and weak instrument.

In summary, we find that cluster-bootstrap  $F$  statistic and the cluster-robust  $F$  statistic, which is equivalent to the “effective”  $F$  (Olea and Pflueger, 2013) in just-identified settings such as this one, are comparable in detecting weak instruments and recommend reporting these statistics in applied settings. We also recommend reporting Anderson-Rubin confidence intervals for the IV coefficient, as it is robust to arbitrarily weak instruments (Andrews, Stock and Sun, 2019; Kang et al., 2021).

## FIGURE A5. COMPARISONS OF $F$ STATISTICS

Cluster-bootstrap  $F$  and (Non-Clustered) Robust Analytic  $F$

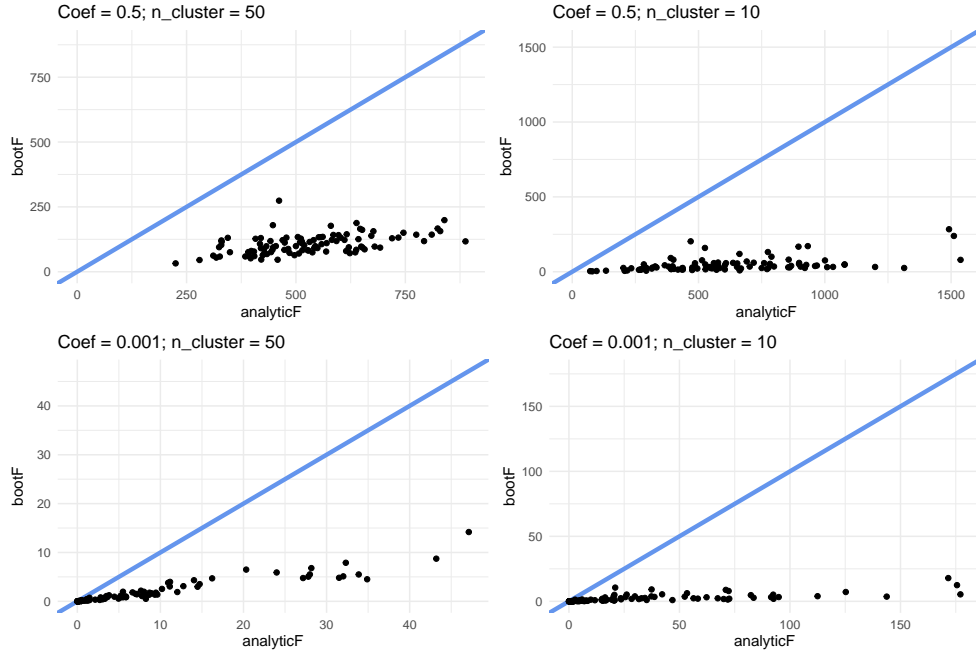

(a) Cluster-bootstrap  $F$  statistic vs. Huber-White (non-clustered)  $F$  statistic

Cluster-bootstrap  $F$  and clustered robust analytic  $F$

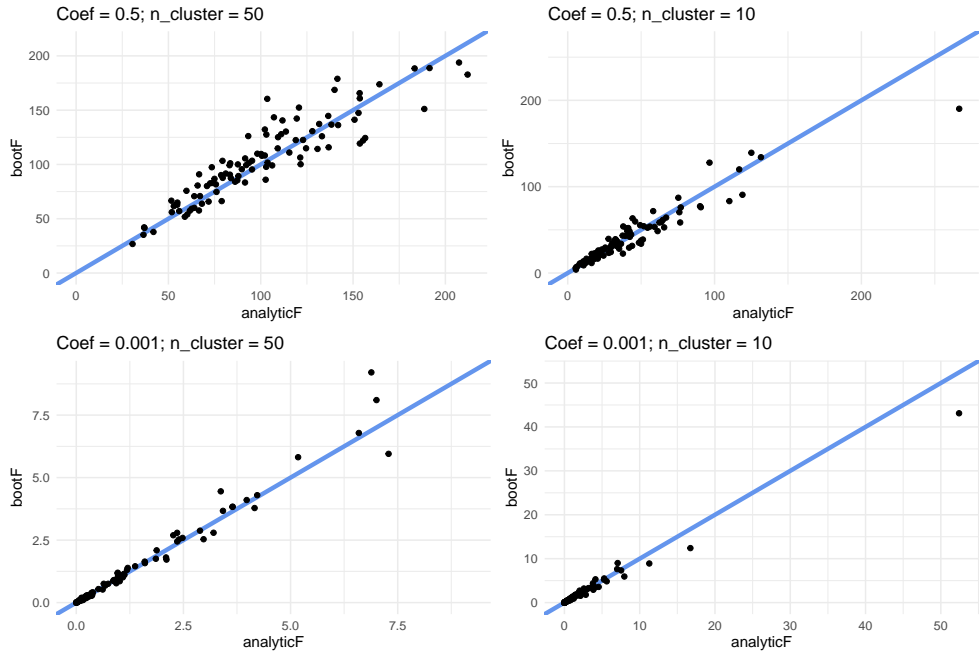

(b) Cluster-bootstrap  $F$  statistic vs. cluster-robust analytic  $F$  statistic ( $F_{Eff}$ )

### A.2.2. Explaining the 2SLS-OLS Discrepancy

In this section, we conduct Monte Carlo exercises to explore potential causes of the discrepancy between 2SLS and OLS estimates observed in the replication data. We consider three causes: (1) violations of the exclusion restriction (A2), (2) publication bias, and (3) heterogeneous treatment effects (HTE). Below is our data-generating process (DGP):

$$\begin{aligned}
y_i &= 5 + \beta_i x_i + \mu z_i + u_i + b_i \\
x_i^* &= \delta_i z_i + (1 - \delta_i) a_i + 0.2 v_i \quad \text{and} \quad \delta_i = \max(\min(\kappa_i \pi_i, 1), 0) \\
x_i &= x_i^*, \quad z_i \stackrel{i.i.d.}{\sim} N(0, 2) \quad (\text{continuous-continuous case}) \\
\text{or} \quad x_i &= 1\{x_i^* > 0\}, \quad z_i \stackrel{i.i.d.}{\sim} \text{Bern}(0.5) \quad (\text{binary-binary case})
\end{aligned}$$

in which  $z$  is the instrument,  $x$  is the treatment, and  $y$  is the outcome. We consider two scenarios: (1) both  $x$  and  $z$  are continuous, and (2) both are binary. Correlated errors  $\begin{bmatrix} u_i \\ v_i \end{bmatrix} \stackrel{i.i.d.}{\sim} N\left(\begin{bmatrix} 0 \\ 0 \end{bmatrix}, \begin{bmatrix} 1 & 0.5 \\ 0.5 & 1 \end{bmatrix}\right)$ ;  $a_i \stackrel{i.i.d.}{\sim} N(0, 1)$ ,  $b_i \stackrel{i.i.d.}{\sim} N(0, 1)$  are i.i.d. errors. We use  $\kappa$  to control the strength of the instrument. HTE can be generated by  $\begin{bmatrix} \beta_i \\ \pi_i \end{bmatrix} \stackrel{i.i.d.}{\sim} N\left(\begin{bmatrix} 2 \\ 1 \end{bmatrix}, \sigma_h^2 \begin{bmatrix} 1 & \lambda \\ \lambda & 0.5 \end{bmatrix}\right)$ , in which  $\sigma_h$  controls the amount of heterogeneity in  $\beta_i$  and  $\pi_i$  while  $\lambda$  controls the correlation between the first stage and reduced form coefficients.  $\delta_i$  is limited to be in  $[0, 1]$ . When  $\lambda > 0$ , it means that a unit's treatment effect is positively correlated with its responsiveness to the IV.<sup>A1</sup> The sample size is fixed at 200.

Under constant treatment effect ( $\sigma_h = 0$ ) and with a valid instrument ( $\mu = 0$ ), the expected value of  $\hat{\beta}_{2SLS}/\hat{\beta}_{OLS}$  is 0.74 for the continuous-continuous case and 0.57 for the binary-binary case. We consider four scenarios sequentially:

1. Violations of Assumption 2 are captured by  $\mu \neq 0$  (failure of the exclusion restriction).
2. Publication bias can be simulated by dropping the cases in which the 2SLS estimates are statistically insignificant at the 5% using a conventional  $t$  test.
3. HTE is generated by setting  $\sigma_h = 0.05$  and  $\lambda = 0.7$ , i.e.,  $\beta_i$  and  $\pi_i$  are highly correlated.
4. The combination of HTE and publication bias.

<sup>A1</sup>For example, under selection-on-gains type settings, which are typically considered in generalized Roy models underlying MTE approaches to IV.

FIGURE A6. CONSEQUENCES OF EXCLUSION RESTRICTION FAILURE  
UNDER CONSTANT EFFECT

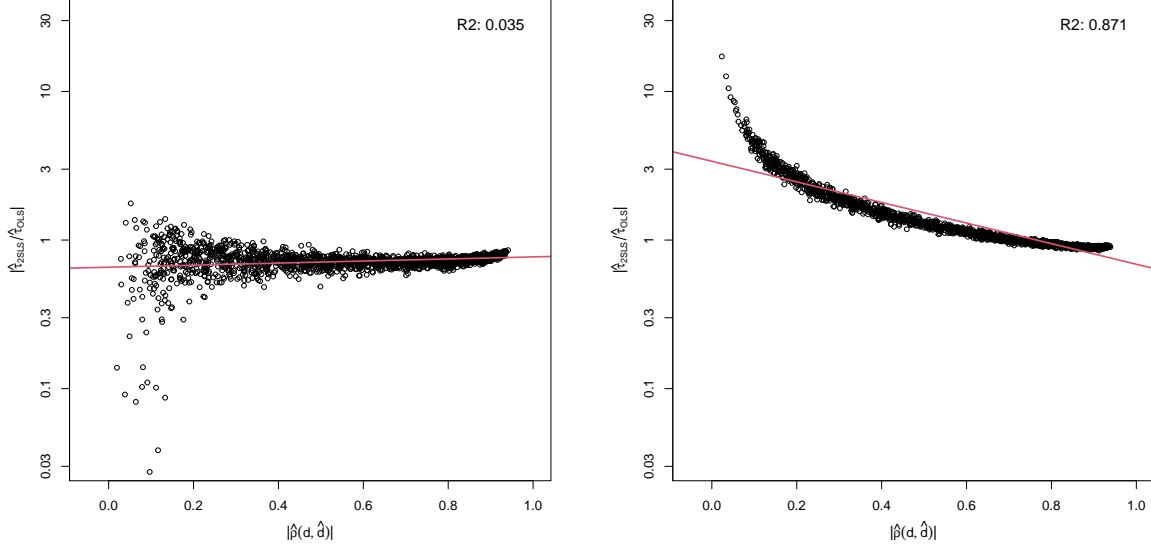

(a) Continuous-Continuous Case: w/o and w/ exclusion restriction failure

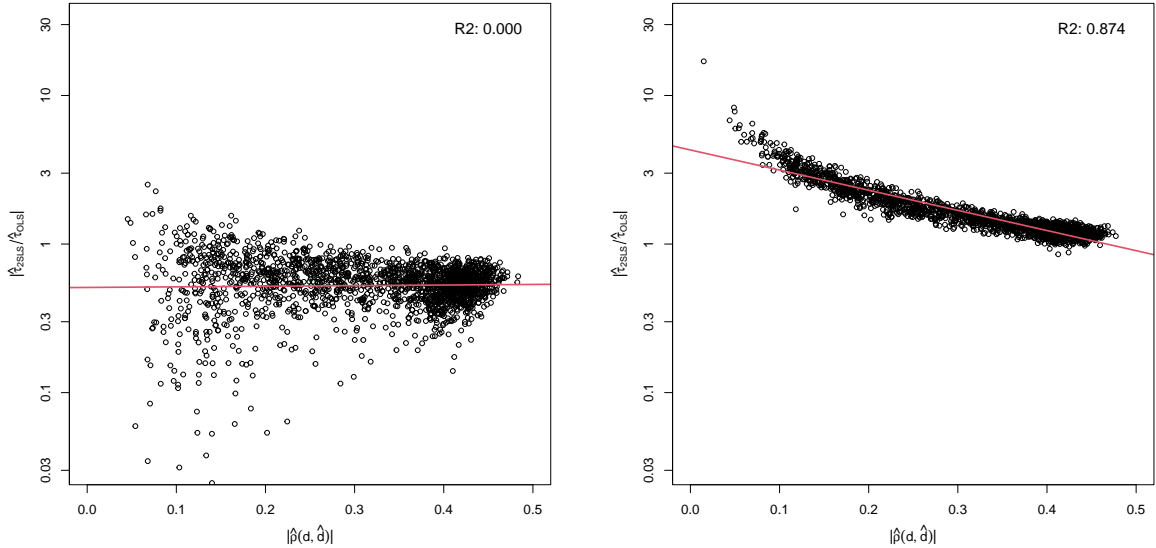

(b) Binary-Binary Case: w/o and w/ exclusion restriction failure

**Violating Assumption 2.** The results for Scenario 1 are shown in Figure A6. Each dot represents one simulated sample. Figure A6 shows that, in both continuous-continuous and binary-binary setups, when the treatment effect is constant ( $\beta_i = \beta, \pi_i = \pi$ ), in expectation, there is no mechanical negative relationship between the correlation coefficient between  $d$  and  $\hat{d}$  and the 2SLS-OLS discrepancy (left panels in both subfigures). However, when the exclusion restriction fails, e.g.,  $\mu = 1$  (right panels in both subfigures), a strong negative

correlation appears. These results support our argument in the paper that a weak first stage amplifies the bias from the failure of Assumption 2.

FIGURE A7. CONSEQUENCES OF PUBLICATION BIAS  
UNDER CONSTANT TREATMENT EFFECT

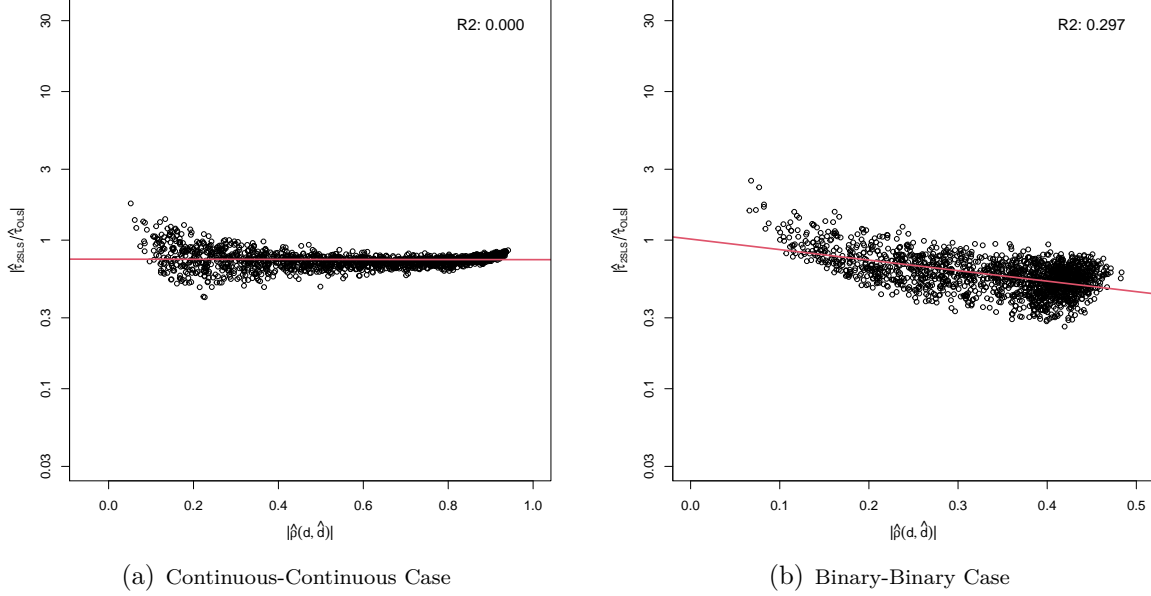

**Publication bias.** Figure A7 illustrates the consequences of publication bias (Scenario 2), where statistically insignificant results are omitted. In the binary-binary case, we observe a moderate negative correlation; however, this correlation is much weaker than those caused by exclusion restriction failures.

**HTE and publication bias.** Finally, we investigate the consequences of HTE (Scenario 3) and its interaction with publication bias (Scenario 4). Figures A8 shows results under HTE, i.e.,  $\sigma_h > 0$  and  $\lambda = 0.7$  ( $\beta_i$  and  $\pi_i$  are highly positively correlated). On the logarithmic scale, the correlation is almost nonexistent (left panels in Figure A8). When we revert to the original scale, we do observe a small to moderate negative correlation in both continuous-continuous and binary-binary cases (figures not shown). When we further introduce publication bias, we begin to see weak negative correlations between the first stage  $\rho$  and the 2SLS-OLS discrepancy on the logarithmic scale, especially in the binary-binary case. However, their magnitudes are much smaller than what we observed in Figure A6 under the exclusion restriction failure. This suggests that the observed strong negative relationship in

FIGURE A8. CONSEQUENCES OF PUBLICATION BIAS UNDER HTE

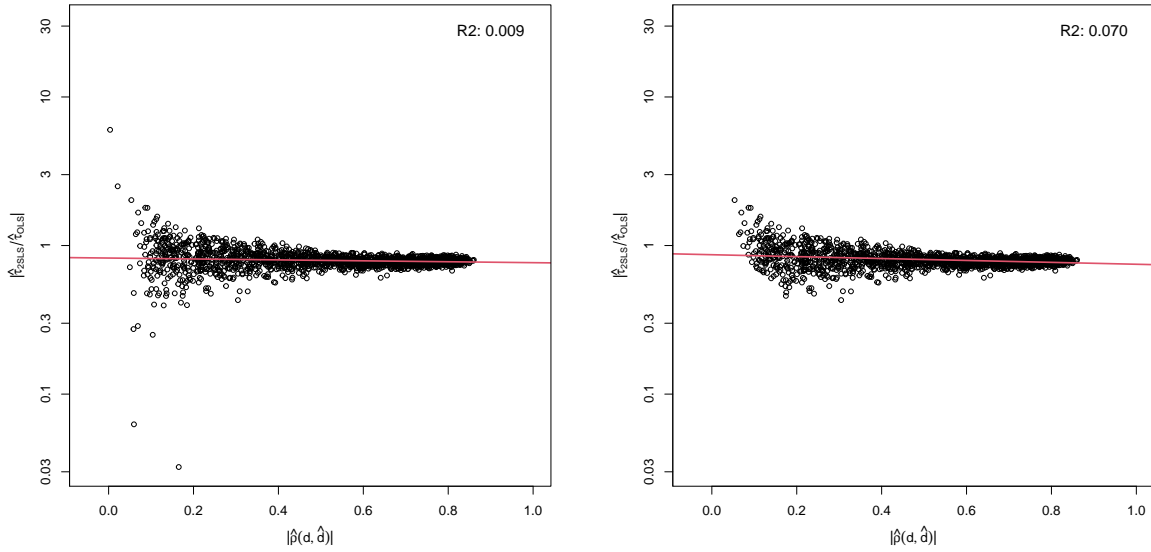

(a) Continuous-Continuous Case: w/o and w/ publication bias

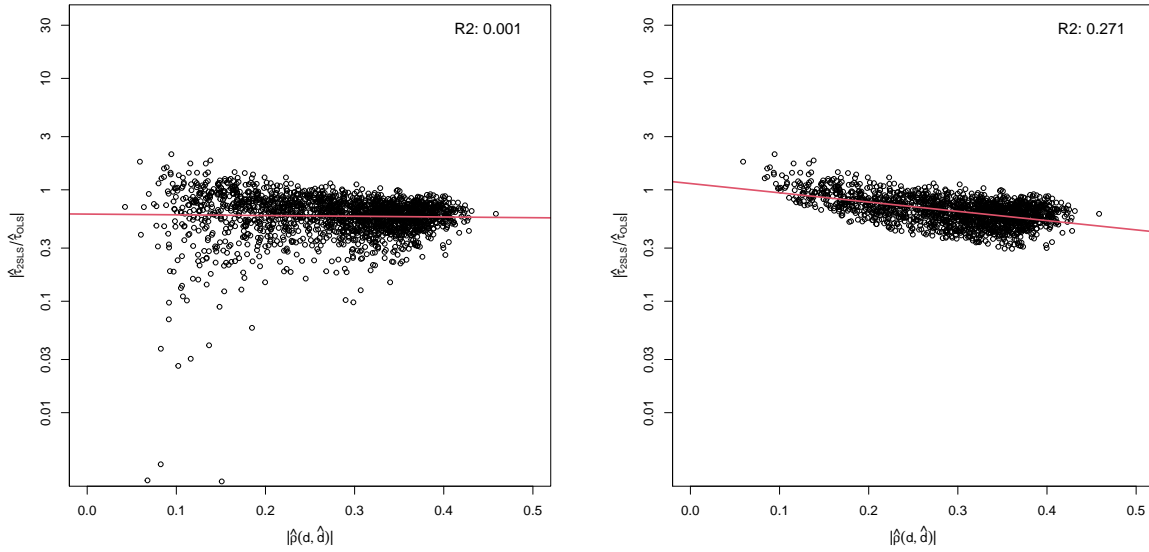

(b) Binary-Binary Case: w/o and w/ publication bias

the paper is unlikely to be solely explained by HTE and different levels of responsiveness to the IV.

In summary, the Monte Carlo exercises demonstrated that the strong negative correlations between the first stage  $\rho$  and the 2SLS-OLS discrepancy are most likely caused by violations of Assumption 2. Other factors, such as publication bias and HTE, may also play a role.

### A.3. Evaluating the Exogeneity Assumption

Assumption 2 is a strong and generally untestable assumption that underlies the validity of the instrument; indeed, researchers typically spend considerable effort arguing for both unconfoundedness and the exclusion restrictions in their particular setting. However, some placebo tests have recently become popular as a way to argue for the validity of identification assumptions in causal designs (Eggers, Tuñón and Dafoe, 2021), especially in observational settings where the choice of IV is guided by detailed domain knowledge. Bound and Jaeger (2000) suggest first using an auxiliary regression on a subsample where the IV is not expected to influence treatment assignment, known as “zero-first-stage” (ZFS) tests. The primary intuition is that in a subsample that one has a strong prior that the first stage is zero—hence, they are “never takers,” to use the language of the LATE framework—the reduced form effect should also be zero if Assumption 2 is satisfied. In other words, motivated by a substantive prior that the first-stage effect of the IV is likely zero for a subsample of the population (henceforth, the “ZFS subsample”), the researcher then proceeds to show that the reduced-form coefficient for the IV (by regression  $Y$  on  $Z$ ) is approximately zero *in the ZFS subsample*, which is suggestive evidence in favor of IV validity. Most observational instruments ought to yield some ZFS subsample based on substantive knowledge of the assignment mechanism.

This style of placebo is particularly popular in studies of historical political economy, where particular historical or geographic features are argued to be valid instruments for treatment assignment, and thus they are unlikely to be driving treatment assignments outside a specific context. For example, Nunn (2008) studies the effects of the slave trade on modern-day development in Africa using sailing distance from each country to the nearest locations of demand for slave labor as an IV for the normalized number of slaves taken. The author then argues that distance to demand locations in the New World are likely to be a valid IV by using a placebo test that the first-stage effect (the IV regressed on the outcome, modern-day GDP) is approximately zero for countries outside Africa, where the posited mechanism (that places close to demand locations exported more slaves only in the transatlantic slave trade) has no traction, thereby providing a candidate ZFS sample. In a related paper, Nunn and Wantchekon (2011) use the same strategy to show that the distance to slave-trade ports do not predict modern-day trust attitudes in the Asiabarometer, while they do in the Afrobarometer (which is the primary study population). Acharya, Blackwell and Sen (2016) perform a similar exercise where they believe that their instrument (cotton suitability) predicts the treatment (slaves per capita) in the Southern States but not the Northern states,

and therefore find that the reduced form effect of cotton suitability on modern-day racial attitudes is approximately zero in the Northern states.

### A.3.1. The ZFS Test and Modified Inference

While this is a useful heuristic check that we advise most observational IV papers adopt, it is an informal test and provides no debiasing procedure to correct potentially biased IV estimates. [Van Kippersluis and Rietveld \(2018\)](#) suggest that the ZFS test can be fruitfully combined with the “plausibly exogenous” method suggested by [Conley, Hansen and Rossi \(2012\)](#) (henceforth, [CHR 2012](#)). To illustrate the method, we first rewrite the IV simultaneous equations in [CHR \(2012\)](#)’s notation:

$$Y = X\beta + Z\gamma + \varepsilon; \quad X = Z\Pi + \nu, \quad (\text{A1})$$

where  $Z$  also enters the structural equation, and the exclusion restriction amounts to a dogmatic prior that  $\gamma = 0$ . [CHR \(2012\)](#) suggest that this assumption can be relaxed, and replaced with a user-specified assumption on a plausible value, range, or distribution for  $\gamma$  depending on the researcher’s beliefs regarding the degree of exclusion restriction violation. They propose three different approaches for inference that involve specifying the range of values for  $\gamma$ , a prior distributional assumption for  $\gamma$ , and a fully Bayesian analysis that requires priors over all model parameters and corresponding parametric distributions. We focus on the second method, which [CHR \(2012\)](#) call the “local to zero” (LTZ) approximation because of its simplicity and transparency. The LTZ approximation considers “local” violations of the exclusion restriction<sup>A2</sup> and requires a prior over  $\gamma$  alone. [CHR \(2012\)](#) show that replacing the standard assumption that  $\gamma = 0$  with the weaker assumption that  $\gamma \sim \mathbb{F}$ , a prior distribution, implies distribution for  $\hat{\beta}$  in Equation [\(A2\)](#).

$$\hat{\beta} \sim^a \mathcal{N}(\beta, \mathbb{V}_{2SLS}) + \mathbf{A}\gamma \quad \text{where } \mathbf{A} \equiv (\mathbf{X}'\mathbf{Z}(\mathbf{Z}'\mathbf{Z})^{-1}\mathbf{Z}'\mathbf{X})^{-1}\mathbf{X}'\mathbf{Z} \quad (\text{A2})$$

$$\hat{\beta} \sim^a \mathcal{N}(\beta + \mathbf{A}\mu_\gamma, \mathbb{V}_{2SLS} + \mathbf{A}\Omega\mathbf{A}') \quad (\text{A3})$$

where the original 2SLS asymptotic distribution is inflated by the additional term. While a simulation-based approach can be used to implement Equation [\(A2\)](#) for an arbitrary distribution for  $\gamma$ , the distribution takes its most convenient form when one uses a Gaussian prior over  $\gamma \sim \mathcal{N}(\mu_\gamma, \Omega_\gamma)$ , which simplifies Equation [\(A2\)](#) to Equation [\(A3\)](#), with a posterior being a Gaussian centered at  $\beta + \mathbf{A}\mu_\gamma$ .

<sup>A2</sup>LTZ asymptotics consider a sequence of constants  $\gamma = C/\sqrt{N}$  for some constant  $C$  and sample size  $N$

CHR (2012) suggest that researchers use domain knowledge to choose  $\mu_\gamma, \Omega_\gamma$ , since they often hold strong priors about instruments anyway (which presumably motivates the choice of the instrument). Van Kippersluis and Rietveld (2018) suggest that a principled method to choose  $\mu_\gamma$  is to estimate Equation (A1) on the ZFS population (wherein  $\Pi$  is assumed to be zero), and use this estimate  $\hat{\gamma}_{ZFS}$  as  $\mu_\gamma$ . This approach combines the informal ZFS test with the plausibly exogenous method in a straightforward manner, and software to implement it is available in both R (accompanying this paper) and STATA (Clarke, 2014). We begin with a simulation-based illustration and illustrate the application of this method to a published empirical paper next.

### A.3.2. Simulation Evidence

In this subsection, we demonstrate the LTZ method when the exclusion restriction is not satisfied. Consider the following DGP,

$$\begin{aligned} Y_i &= \beta_i D_i + \gamma Z_i + \varepsilon_i \\ D_i &= \mathbf{1}\{D_i^* > 0\} \\ D_i^* &= \alpha_i + \pi_i Z_i + \varepsilon_i \end{aligned}$$

in which  $Z_i \sim \text{Bernoulli}(0.5)$  is a binary instrument,  $\pi_i \sim \text{U}[1.5, 2.5]$ ,  $\alpha_i \sim \mathcal{N}(-1, 1)$ ,  $\varepsilon_i \sim \mathcal{N}(0, 1)$ ,  $\beta_i \sim \mathcal{N}(1, 0.25)$ . We generate  $Y_i$  with  $Z_i$  directly entering the structural equation, which allows us to vary the magnitude of the exclusion restriction violation. We then estimate  $\hat{\beta}_{2SLS}$  using conventional 2SLS on this data. As we vary  $\gamma$ ,  $\hat{\beta}_{2SLS}$  is inconsistent for all values except when  $\gamma = 0$ . We set  $\pi = 0$  for the last 20% observations of the simulated data (the ZFS subsample). We then estimate the reduced-form regression on this (known) subsample and use the coefficient as a prior for  $\mu_\gamma$ , and compute the LTZ IV estimate.

Figure A9 shows, unlike the 2SLS estimator (blue), the LTZ estimator (orange) uncovers the true value of  $\beta = 2$  even for large degrees of exclusion restriction violations (large  $|\gamma|$ ).

### A.3.3. A Case Study

We illustrate the diagnostics described above by applying it to the IV analysis in Guiso, Sapienza and Zingales (2016) (henceforth GSZ 2016), who revisit Putnam, Leonardi and Nanetti (1993)'s conjecture that Italian cities that achieved self-government in the Middle Ages have higher modern-day levels of social capital. More specifically, they study the effects

FIGURE A9. IV AND LTZ ESTIMATES FOR VARYING  $\gamma$

LTZ and TSLS coefficients for Exclusion restriction violations of varying severity  
True effect = 2

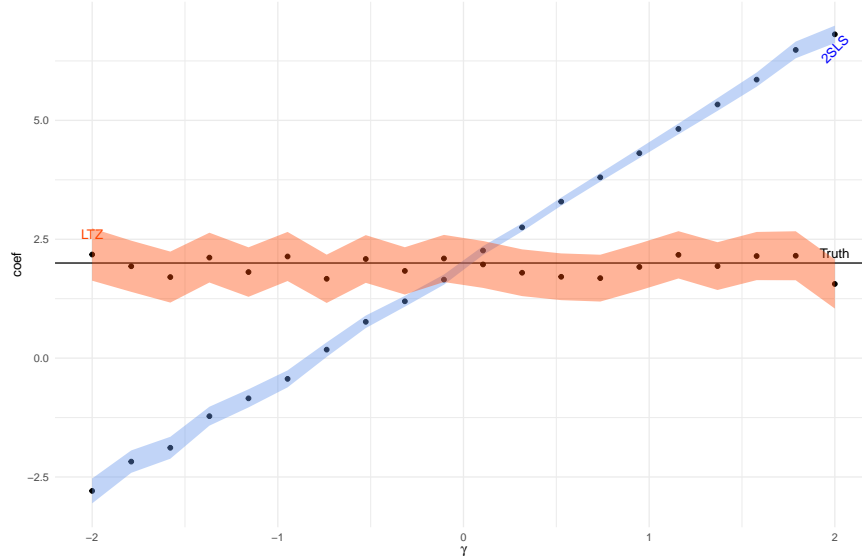

of free city-state status on social capital as measured by the number of non-profits and organ donations per capita, and a measure of whether students cheat in mathematics.

TABLE A1. REPLICATION OF GSZ (2016) TABLE 6  
REDUCED FORM REGRESSIONS

| <i>Outcome Variables</i> | North            |                       | South (ZFS)      |                       |
|--------------------------|------------------|-----------------------|------------------|-----------------------|
|                          | Nonprofit<br>(1) | Organ Donation<br>(2) | Nonprofit<br>(3) | Organ Donation<br>(4) |
| Bishop (IV)              | 1.612<br>(0.219) | 0.472<br>(0.047)      | 0.178<br>(0.137) | 0.189<br>(0.065)      |
| Observations             | 5,357            | 5,535                 | 2,175            | 2,178                 |

**Note:** Bootstrapped SEs are in the parentheses. See Figure A4 in the SM for the original table.

GSZ (2016) use a dummy for whether the city was the seat of a bishop in the Middle Ages, based on historical accounts of coordination preceding commune formation in the Middle Ages as an IV for the “free-city experience” (Section 5). They argue that conditional on a host of geographic covariates, this IV, a bishop seat, influences contemporary social capital solely through its increasing the likelihood of commune formation. As suggestive evidence for the validity of their instrument, they estimate the reduced-form effect of medieval bishop presence of contemporary social capital measures separately in the north (where the IV is conjectured to have an effect) and the south (where it is conjectured to be irrelevant). They

FIGURE A10. TABLE 6 IN [GUIO, SAPIENZA AND ZINGALES \(2016\)](#)

TABLE 6. Validating the instrument.

| <b>A. Regressions of civic capital in the Center–North and in the South</b> |                          |                                   |                                          |                           |                                  |                                         |
|-----------------------------------------------------------------------------|--------------------------|-----------------------------------|------------------------------------------|---------------------------|----------------------------------|-----------------------------------------|
|                                                                             | Center–North sample      |                                   |                                          | South sample              |                                  |                                         |
|                                                                             | (I)<br>Nonprofit<br>org. | (II)<br>Organ<br>donation<br>org. | (III)<br>Cheating<br>in mathe-<br>matics | (IV)<br>Nonprofit<br>org. | (V)<br>Organ<br>donation<br>org. | (VI)<br>Cheating<br>in mathe-<br>matics |
| Ease of coordination                                                        | 1.61**<br>(0.219)        | 0.47***<br>(0.047)                | −0.66***<br>(0.118)                      | 0.18<br>(0.137)           | 0.19***<br>(0.065)               | −0.04<br>(0.309)                        |
| Elevation                                                                   | 1.93***<br>(0.475)       | −0.25***<br>(0.062)               | 0.94**<br>(0.441)                        | 1.43***<br>(0.257)        | −0.04<br>(0.083)                 | 0.72<br>(0.541)                         |
| Max difference in<br>elevation                                              | 1.35***<br>(0.219)       | 0.01<br>(0.026)                   | 0.26*<br>(0.143)                         | −0.08<br>(0.084)          | −0.05*<br>(0.029)                | 0.06<br>(0.145)                         |
| City is on the coast                                                        | −0.27<br>(0.264)         | −0.08*<br>(0.046)                 | 0.03<br>(0.119)                          | 0.23**<br>(0.115)         | −0.02<br>(0.044)                 | 0.13<br>(0.108)                         |
| City more than 5 km<br>from the coast                                       | 1.10*<br>(0.634)         | 0.07<br>(0.072)                   | −0.21<br>(0.227)                         | 0.02<br>(0.143)           | −0.03<br>(0.048)                 | 1.46<br>(1.098)                         |
| Current population                                                          | −3.38***<br>(1.886)      | 1.48***<br>(0.290)                | −1.85***<br>(0.523)                      | −9.11***<br>(2.242)       | 1.10*<br>(0.582)                 | −3.50<br>(2.849)                        |
| Current population<br>squared                                               | 1.03<br>(1.423)          | −1.12***<br>(0.218)               | 1.87***<br>(0.480)                       | 6.23***<br>(1.924)        | −0.86*<br>(0.469)                | 4.47<br>(2.816)                         |
| Gini income<br>inequality index                                             | 0.08<br>(0.449)          | 0.04<br>(0.076)                   | 0.04<br>(0.438)                          | 3.49**<br>(1.505)         | 2.05***<br>(0.547)               | −21.66***<br>(5.646)                    |
| Gini inequality index<br>of land ownership                                  | 9.83***<br>(1.883)       | 2.17***<br>(0.377)                | −8.61***<br>(2.382)                      | 1.61***<br>(0.351)        | 0.35***<br>(0.098)               | 1.75<br>(1.330)                         |
| Observations                                                                | 5,357                    | 5,535                             | 1,911                                    | 2,175                     | 2,178                            | 1,210                                   |
| $R^2$                                                                       | 0.083                    | 0.587                             | 0.023                                    | 0.329                     | 0.574                            | 0.027                                   |

**Note:** “Ease of coordination” is the IV “Bishop in city.” We replicated columns (I), (II), (IV), and (V).

fail to reject the null of no effects in the south, conclude that the IV appears to have face validity, and proceed to use bishop’s presence as an IV for their IV estimates.

We begin by calculating the first-stage partial  $F$  statistic based on bootstrapped SEs for the north sample, which is 67.3. Because there were no “free cities” in the south, the  $F$  statistic for the south is zero by definition. We then replicate their reduced-form estimates in Table A1. The separate north and south reduced-form estimates in GSZ (2016) can be readily used for the LTZ test described above. The authors substantively believe that the south is a ZFS sample where bishop presence is irrelevant for treatment assignment,<sup>A3</sup> we can use the reduced-form estimates of 0.178 and 0.189 in the south for non-profits per capita and organ donation (columns 3-4 in Table A1) as the prior  $\mu_\gamma$  for the direct effect of the IV on the

<sup>A3</sup>The authors claim this indirectly by reporting the reduced form effects separately for the north and south subsamples in Table 6, and state that since the reduced form is attenuated in the south, this justifies the use of bishop presence as an IV (p. 1427).

FIGURE A11. IV COEFFICIENTS FOR NON-PROFITS AND ORGAN DONATION

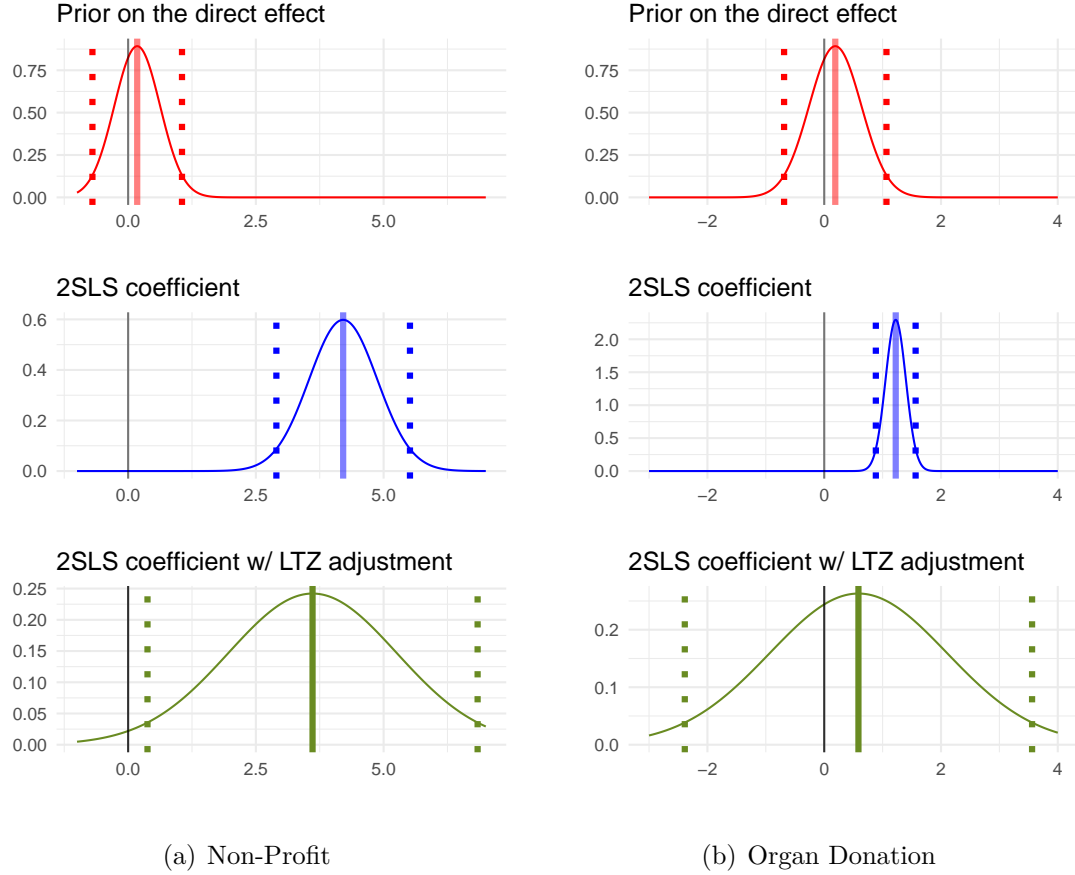

outcome. Finally, we report the analytic, bootstrap, and LTZ IV results in Figure A11. We find that conventional robust SEs understate the uncertainty of the estimates relative to the bootstrap and that accounting for direct effect using LTZ attenuates GSZ (2016)'s estimates somewhat and substantially increases the SE of the estimate for the non-profit outcome. For organ donation, however, where we suspect a violation of Assumption 2 because the reduced form effect is statistically distinguishable from zero, the use of the LTZ method to account for this exclusion restriction violation yields a smaller and substantially more uncertain estimate whose CI contains 0. This example shows how researchers may take advantage of the ZFS test and the LTZ technique to gauge the robustness of their findings based on an IV strategy.

## A.4. Summary of Replicated Papers

TABLE A2. SUMMARY OF REPLICATED PAPERS

| Paper                               | Instrument                                      | Treatment                                              | Outcome                                      | IV Type                                     | Justification for IV Validity                                                                                                                                                                                                                                                                          |
|-------------------------------------|-------------------------------------------------|--------------------------------------------------------|----------------------------------------------|---------------------------------------------|--------------------------------------------------------------------------------------------------------------------------------------------------------------------------------------------------------------------------------------------------------------------------------------------------------|
| APSR                                |                                                 |                                                        |                                              |                                             |                                                                                                                                                                                                                                                                                                        |
| Gerber, Huber and Washington (2010) | Being sent mail                                 | Aligning party identification with latent partisanship | Voting and party alignment scale             | Experiment                                  | NA                                                                                                                                                                                                                                                                                                     |
| Meredith (2013)                     | Governors home county                           | Democratic governor                                    | Down-ballot Democratic candidates vote share | Theory (Other)                              | “The validity of the instruments hinges on the assumption that, conditional on the control variables, coattail effects are the only channel through which the place of birth or residence of a party’s gubernatorial candidate affects the vote shares received by its down-ballot candidates.”(p.745) |
| Blattman, Hartman and Blair (2014)  | Assignment to treatment blocks                  | Mass education campaign for dispute resolution         | Serious land dispute                         | Experiment                                  | NA                                                                                                                                                                                                                                                                                                     |
| Laitin and Ramachandran (2016)      | Geographic distance from the origins of writing | Language choice                                        | Human development index                      | Theory (Geography)                          | “[T]he distance from these sites of invention should have no independent impact on socioeconomic development today, except through the channel of affecting the probability of possessing a writing tradition.” (p. 470)                                                                               |
| Ritter and Conrad (2016)            | Rainfall                                        | Mobilized dissent                                      | Repression                                   | Theory (Weather)                            | “[R]ainfall is an exogenous predictor of dissent onset, meeting the key criteria for the instrumental analysis to allow for causal inference.”(p.89)                                                                                                                                                   |
| Croke et al. (2016)                 | Access to the secondary education               | Education attainment                                   | Political participation                      | Rules & policy changes (Change in exposure) | “There are, however, good reasons to believe that the secondary education reform only affects participation through its effect on educational attainment.”(p.592)                                                                                                                                      |
| Dower et al. (2018)                 | Level of serfdom                                | Frequency of unrest                                    | Peasant representation and unrest            | Theory (History)                            | “After conditioning on these covariates, we are left with that portion of serfdom largely determined by idiosyncratic variation in land grants to the nobility decades or centuries before the zemstvo reform of 1864.” (p. 133)                                                                       |

|                                    |                                                                              |                                                                        |                                   |                                             |                                                                                                                                                                                                                                                                                                                                  |
|------------------------------------|------------------------------------------------------------------------------|------------------------------------------------------------------------|-----------------------------------|---------------------------------------------|----------------------------------------------------------------------------------------------------------------------------------------------------------------------------------------------------------------------------------------------------------------------------------------------------------------------------------|
| Dower et al. (2018)                | Religious polarization                                                       | Frequency of unrest                                                    | Peasant representation and unrest | Theory (History)                            | “After conditioning on these covariates, we are left with that portion of serfdom largely determined by idiosyncratic variation in land grants to the nobility decades or centuries before the zemstvo reform of 1864.” (p. 133)                                                                                                 |
| Nellis and Siddiqui (2018)         | Narrow victory by secular parties in a district                              | The proportion of MNA seats in a district won by secularist candidates | Religious violence                | Theory (Election)                           | “Our identifying assumption is that the outcomes of such close elections are as good as randomly decided.” (p. 50)                                                                                                                                                                                                               |
| Kapoor and Magesan (2018)          | Changes in entry costs.                                                      | Number of independent candidates                                       | Voter turnout                     | Rules & policy changes (Change in exposure) | “It is worth reiterating that the deposit increases had nothing to do with historical differences in voter and candidate participation across reserved and open constituencies.” (p. 681)                                                                                                                                        |
| Colantone and Stanig (2018a)       | Imports from China to the United States $\times$ local industrial structure  | Regional-level import shock from China                                 | Leave support in Brexit           | Econometrics (Interaction)                  | “[The ]instrument is meant to capture the variation in Chinese imports, which is due to the exogenous changes in supply conditions in China, rather than to domestic factors in the United Kingdom that could be correlated with electoral outcomes.” (p. 206)                                                                   |
| Hager, Krakowski and Schaub (2019) | Distance to the nearest location where armored military vehicles were stolen | Ethnic riots (destruction)                                             | Prosocial behavior                | Theory (Other)                              | “[W]e present a falsification test which corroborates that the instrument is unrelated to prosocial behavior in a sample of 136 nearby villages, thus underlining the exclusion restriction.” (p. 1037)                                                                                                                          |
| Baccini and Weymouth (2021)        | Bartik instrument                                                            | Manufacturing Layoffs                                                  | Change of Democratic Vote Share   | Econometrics (Interaction)                  | “Since layoffs are not randomly assigned, we develop an instrumental variables strategy using shift-share methodology (Bartik 1991) derived from national layoff shocks, weighted by initial county-level employment.”(p.550)                                                                                                    |
| Hager and Krakowski (2022)         | Number of corrupted Catholic priests                                         | Number of secret police officers                                       | Resistance                        | Theory (History)                            | “In the early days of the regime, the secret polices ability to servile citizens depended critically on the cooperation of the Catholic Church...Importantly, the corruptibility of priests was plausibly exogenous: priests were sent to municipalities by the Catholic Church, often when another priest had retired.” (p.565) |

|                                     |                                                                           |                                                                             |                                                      |                                     |                                                                                                                                                                                                                                                                                                                   |
|-------------------------------------|---------------------------------------------------------------------------|-----------------------------------------------------------------------------|------------------------------------------------------|-------------------------------------|-------------------------------------------------------------------------------------------------------------------------------------------------------------------------------------------------------------------------------------------------------------------------------------------------------------------|
| Kuipers and Sahn (2022)             | Statewide assignment mandate                                              | Civil service reform                                                        | Descriptive representation on an unrestricted sample | Rules & policy changes (Assignment) | “First, we assume that state-level mandates are a strong instrument for city adoption; we verify the strength of the instrument in the main presentation of the results. The exclusion restriction, which is untestable, seems a reasonable assumption in our case.”(p.9)                                         |
| AJPS                                |                                                                           |                                                                             |                                                      |                                     |                                                                                                                                                                                                                                                                                                                   |
| Kocher, Pepinsky and Kalyvas (2011) | Past insurgent control                                                    | Aerial bombing                                                              | Changes in local control                             | Theory (Other)                      | “Because instrumental variables require only conditional independence between instruments and the error term, we need only assume that there are no unobserved hamlet-specific variables that affected insurgent control in July, August, and December 1969, but not in September of that year as well.” (p. 212) |
| Vernby (2013)                       | Immigration Inflow 19401950; immigration Inflow 19601967                  | Share of noncitizens in the electorate                                      | Municipal education and social spending              | Theory (History)                    | “Furthermore, it is unlikely that the initial locations of these refugees were affected by the level of local public services, suggesting that the instrument is also valid.” (p. 25)                                                                                                                             |
| Tajima (2013)                       | Distance to health station                                                | Distance to police posts (as a proxy for exposure to military intervention) | Incidence of communal violence                       | Theory (Geography)                  | “According to a Health Department official, primary health stations must be located in every subdistrict at their population centers, regardless of the propensity for violence of those locations” (p. 112)                                                                                                      |
| De La O (2013)                      | Random assignment to early coverage                                       | Early coverage of Conditional Cash Transfer                                 | Incumbent party’s vote share                         | Experiment                          | NA                                                                                                                                                                                                                                                                                                                |
| McClendon (2014)                    | Assignment to treatment                                                   | Reading social esteem promising email                                       | Participation in LGBTQ events                        | Experiment                          | NA                                                                                                                                                                                                                                                                                                                |
| Barth, Finseraas and Moene (2015)   | Adjusted bargaining coverage and effective number of union confederations | Wage inequality                                                             | Welfare support                                      | Theory (Other)                      | “Yet conditional on union density and country fixed effects, we argue that certain properties of the bargaining system are likely to affect wages, but not union involvement in politics.” (p. 574)                                                                                                               |

|                                 |                                                                   |                                             |                                             |                                   |                                                                                                                                                                                                                                                              |
|---------------------------------|-------------------------------------------------------------------|---------------------------------------------|---------------------------------------------|-----------------------------------|--------------------------------------------------------------------------------------------------------------------------------------------------------------------------------------------------------------------------------------------------------------|
| Stokes (2016)                   | Wind speed                                                        | Turbine location                            | Vote turnout                                | Theory (Climate)                  | “Wind speed is theoretically orthogonal to precinct boundaries but predicts the placement of wind turbine locations.” (p. 965)                                                                                                                               |
| Coppock and Green (2016)        | Mailing showing 2005 Vote                                         | Voting in November 2007 municipal elections | Voting in the 2008 presidential primary     | Experiment                        | NA                                                                                                                                                                                                                                                           |
| Trounstone (2016)               | The number of waterways in a city combined with logged population | Racial segregation                          | Direct general expenditures                 | Theory (Geography)                | “I focus on waterways (including large streams and rivers), which vary in number across cities and are arguably exogenous to segregation and spending.” (p. 717)                                                                                             |
| Carnegie and Marinov (2017)     | Being a former colony of one of the Council members               | Foreign aid                                 | CIRI Human Empowerment index                | Theory (History)                  | “In 1965, the EU stipulated that countries would hold the presidency for 6 months at a time [...] and would rotate alphabetically according to each member states name as spelled in its own language. ” (p. 676)                                            |
| Zhu (2017)                      | Weighted geographic distance from economic centers                | MNC activity                                | Corruption                                  | Theory (Geography)                | “This instrumental variable (IV) is rooted in the gravity models of international trade and FDI flows.” (p. 90)                                                                                                                                              |
| Rueda (2017)                    | The size of the polling station                                   | Actual polling place size                   | Citizens’ reports of electoral manipulation | Rules & policy changes (Fuzzy RD) | “The institutional rule predicts sharp reductions in the size of the average polling station of a municipality every time the number of registered voters reaches a multiple of the maximum number of voters allowed to vote in a polling station.” (p. 173) |
| Lelkes, Sood and Iyengar (2017) | State-level ROW index                                             | Number of providers                         | Affective polarization (partisan hostility) | Theory (Other)                    | “[A]n index of state regulation of right-of-way laws strongly predicts the number of providers in a county, which, as we discuss later, is a good proxy for broadband uptake.” (p. 4).                                                                       |
| Goldstein and You (2017)        | Direct flight from city to Washington DC                          | Lobbying spending                           | Total earmarks or grants awarded            | Theory (Other)                    | “The existence of a direct flight captures the convenience of travel to Washington, DC, from each city.” (p. 865)                                                                                                                                            |

|                                       |                                                                             |                                                                                        |                                     |                                   |                                                                                                                                                                                                                                                                            |
|---------------------------------------|-----------------------------------------------------------------------------|----------------------------------------------------------------------------------------|-------------------------------------|-----------------------------------|----------------------------------------------------------------------------------------------------------------------------------------------------------------------------------------------------------------------------------------------------------------------------|
| Spenkuch and Tillmann (2018)          | Individual princes decisions concerning whether to adopt Protestantism      | Religion of voters living in the same areas more than three and a half centuries later | Nazi vote share                     | Theory (History)                  | “The historical record, however, suggests that princes decisions may plausibly satisfy this exogeneity assumption, especially after controlling for economic conditions at the end of the Weimar Republic as well as all factors known to have influenced rulers.” (p. 27) |
| Colantone and Stanig (2018b)          | Chinese imports to the United States $\times$ regional industrial structure | Regional import shock from China                                                       | Economic nationalism                | Econometrics (Interaction)        | “This instrument is meant to capture the variation in Chinese imports due to exogenous changes in supply conditions in China, rather than to domestic factors that could be correlated with electoral outcomes.” (p. 6)                                                    |
| Hager and Hilbig (2019)               | Mean elevation                                                              | Equitable inheritance customs                                                          | Female representation               | Theory (Geography; History)       | “Rivers are exogenous, but no longer should have a strong effect on inequality other than through the treatment.” (p. 767)                                                                                                                                                 |
| Hager and Hilbig (2019)               | Distance to rivers                                                          | Equitable inheritance customs                                                          | Female representation               | Theory (Geography; History)       | “Rivers are exogenous, but no longer should have a strong effect on inequality other than through the treatment.” (p. 767)                                                                                                                                                 |
| Chong et al. (2019)                   | Treatment assignment in get-out-to-vote campaigns                           | Actual proportion of households treated in the locality                                | Voted in 2013 presidential election | Experiment                        | NA                                                                                                                                                                                                                                                                         |
| Kim (2019)                            | Population threshold                                                        | Democratic institutions                                                                | Women political engagement          | Rules & policy changes (Fuzzy RD) | “[L]ocalities with a population greater than 1,500 must create a municipal council [...] whereas those with a population below that threshold were free to choose between the status quo direct democracy and representative democracy.” (p. 6).                           |
| Sexton, Wellhausen and Findley (2019) | Soldier fatalities                                                          | Health budget                                                                          | Welfare outcome                     | Theory (Other)                    | “We substantiate [the exclusion restriction] below by ruling out the key alternative channel that local insecurity could affect citizens use of health services.” (p. 359)                                                                                                 |
| López-Moctezuma et al. (2022)         | Assignment to treatment                                                     | Town-hall meetings                                                                     | Voting behavior                     | Experiment                        | NA                                                                                                                                                                                                                                                                         |

|                                      |                                                                         |                                                     |                                    |                           |                                                                                                                                                                                                                                                                                                                                                                                                                                            |
|--------------------------------------|-------------------------------------------------------------------------|-----------------------------------------------------|------------------------------------|---------------------------|--------------------------------------------------------------------------------------------------------------------------------------------------------------------------------------------------------------------------------------------------------------------------------------------------------------------------------------------------------------------------------------------------------------------------------------------|
| Blair, Di Salvatore and Smidt (2022) | Average fragmentation of all ongoing PKO mandates                       | Fragmentation of any given PKO mandate              | Process performance                | Theory (Other)            | “We view the first of these assumptions as mostly uncontroversial. As discussed above, most PKO mandates are only loosely tailored to conditions in their host countries. It is highly unlikely that the mandates of all other PKOs in Africa are tailored to the host country conditions of any given PKO. This should mitigate independence concerns.” (p.11)                                                                            |
| Hong, Park and Yang (2022)           | Geographic terrain elevation and slope                                  | NVM subsidies                                       | Parks vote share in 2012           | Theory (Geography)        | “The logic behind this choice is as follows: each villages performance in the NVM is evaluated based on their baseline conditions. Therefore, an unfavorable terrain before the movement likely indicates an initial lack of infrastructure in a poorer environment, and thus gives a village an advantageous benchmark from which to generate a notable and visible improvement within a short period compared to other villages.” (p.11) |
| Wood and Grose (2022)                | Random audit                                                            | Incumbent found to have campaign finance violations | Legislator retired                 | Experiment                | NA                                                                                                                                                                                                                                                                                                                                                                                                                                         |
| JOP                                  |                                                                         |                                                     |                                    |                           |                                                                                                                                                                                                                                                                                                                                                                                                                                            |
| Gehlbach and Keefer (2012)           | Whether the first ruler in a nondemocratic episode is a military leader | Age of ruling party less leader years in office     | Private investment/GDP             | Theory                    | “[D]ictators who come to power with the backing of the military require less popular support to remain in power and are therefore less likely to promote private investment by allowing supporters to organize.” (p. 628)                                                                                                                                                                                                                  |
| Healy and Malhotra (2013)            | Whether the younger sibling is a sister                                 | The share of a respondents siblings who are female  | 1973 gender-role attitude          | Theory (Others – Biology) | “However, under Assumption 1, all siblings have an impact only through the overall gender makeup of the household.” (p. 1027)                                                                                                                                                                                                                                                                                                              |
| Dube and Naidu (2015)                | US military aid to countries outside of Latin America                   | US military aid to Colombia                         | The number of paramilitary attacks | Theory (Diffusion)        | “The instrument is valid since US funding to the rest of the world is determined by the broad geopolitical outlook of the American government, reflecting factors such as the party of the president or other major world events, and can thus be considered exogenous to the conflict in Colombia.”(p.256)                                                                                                                                |

|                                     |                                                                                                                       |                                                         |                                          |                                  |                                                                                                                                                                                                                                                                                           |
|-------------------------------------|-----------------------------------------------------------------------------------------------------------------------|---------------------------------------------------------|------------------------------------------|----------------------------------|-------------------------------------------------------------------------------------------------------------------------------------------------------------------------------------------------------------------------------------------------------------------------------------------|
| Flores-Macias and Kreps (2013)      | Lagged values of country's energy production                                                                          | Trade volume                                            | Foreign policy convergence               | Theory (Other)                   | "The logic is that trade and trade salience in Africa and Latin America are significantly related to countries energy production, but there is no reason to believe that either of them is correlated with the error term in the equation predicting foreign policy convergence" (p. 365) |
| Charron and Lapuente (2013)         | Consolidation of clientelistic networks in regions where rulers have historically less constraints to their decisions | Clientelism                                             | Quality of government                    | Theory (History)                 | "[W]e also find that constraints are directly correlated with current regional institutional quality (yet in his analysis regional GDP and GDP growth are used), thus rendering it an imperfect instrument for clientelism"(p.576)                                                        |
| Kriner and Schickler (2014)         | Number of days Congress is in session                                                                                 | Committee investigations                                | Presidential approval                    | Theory (Other)                   | "[T]here is no theoretical reason drawn from existing literatures to expect the calendar to be independently correlated with presidential approval." (p. 525)                                                                                                                             |
| Lorentzen, Landry and Yasuda (2014) | Large firm dominance in 1999                                                                                          | Large firm dominance in 2007                            | Pollution information transparency index | Econometrics (Lagged treatment)  | "[The instrument was measured] well before transparency reforms were a major focus of discussion." (p. 187)                                                                                                                                                                               |
| Dietrich and Wright (2015)          | Constructed "internal" excluded instrument                                                                            | Economic aid                                            | Transitions to multipartyism             | Econometrics (Lewbel instrument) | "[We]show that the excluded instruments are generally uncorrelated with alternative channels through which they might influence the outcome variables." (p. 223)                                                                                                                          |
| Feigenbaum and Hall (2015)          | Chinese exports to other economies × local exposure                                                                   | Localized trade shocks in congressional districts       | Trade score                              | Econometrics (Interaction)       | "[We] use an instrument that depends [...] on Chinese import growth to other rich, Western economies" and "the lagged version is unaffected by Chinese trade shock." (p.1019)                                                                                                             |
| Alt, Marshall and Lassen (2016)     | Assignment to receiving an aggregate unemployment forecast                                                            | Unemployment expectations                               | Vote intention                           | Experiment                       | NA                                                                                                                                                                                                                                                                                        |
| Johns and Pelc (2016)               | Trade stake of the rest of the world                                                                                  | The number of other countries that became third parties | Becoming a third party                   | Theory (Other)                   | "[E]ach states participation decision is not directly affected by the trade stake of other countries. The trade stake of other countries matters only to the extent that it shapes a players belief about how other countries will behave." (p. 99)                                       |

|                                    |                                                                            |                                                         |                                      |                                             |                                                                                                                                                                                                                                                                                                                                                                                                                                                       |
|------------------------------------|----------------------------------------------------------------------------|---------------------------------------------------------|--------------------------------------|---------------------------------------------|-------------------------------------------------------------------------------------------------------------------------------------------------------------------------------------------------------------------------------------------------------------------------------------------------------------------------------------------------------------------------------------------------------------------------------------------------------|
| Acharya, Blackwell and Sen (2016)  | Measures of the environmental suitability for growing cotton               | Slave proportion in 1860                                | proportion Democrat                  | Theory (History)                            | “We present results from this analysis showing that, outside the South, the relationship between cotton suitability and political attitudes is either very small or in the opposite direction as in the South.” (p. 628)                                                                                                                                                                                                                              |
| Schleiter and Tavits (2016)        | Prime Minister dissolution power                                           | Opportunistic election calling                          | Vote share of Prime Minister’s party | Theory (Other)                              | “The instrument correlates directly with the treatment of interestopportunistic election callingwithout being linked to anticipated incumbent electoral performance.” (p. 840)                                                                                                                                                                                                                                                                        |
| Henderson and Brooks (2016)        | Rain around Election day                                                   | Democratic vote margins                                 | Incumbent roll call positioning      | Theory (Weather)                            | “Rain several days before an election may dampen the willingness to make plans, arrange transportation, and schedule time off work to go to the polls.”(p.657)                                                                                                                                                                                                                                                                                        |
| Henderson and Brooks (2016)        | Rain around Election weekend                                               | Democratic vote margins                                 | Incumbent roll call positioning      | Theory (Weather)                            | “Rain several days before an election may dampen the willingness to make plans, arrange transportation, and schedule time off work to go to the polls.”(p.657)                                                                                                                                                                                                                                                                                        |
| Charron et al. (2017)              | Proportion of Protestant residents in a region; aggregate literacy in 1880 | More developed bureaucracy                              | Percent of single bidders            | Theory (History)                            | “[C]ross-country data show that, while the least corrupted countries in the world all have had near universal literacy for decades, other countries considered highly corrupt, [...] have, for the entire postwar era, also been some of the most highly literate places in the world.” (p.97)                                                                                                                                                        |
| West (2017)                        | IEM (prediction market) price                                              | Obama win                                               | Policy efficacy                      | Theory (Other)                              | “The identifying assumption is that there is no unobservable factor that simultaneously affects black (female) political efficacy and perceptions of the likelihood of an Obama (Clinton) victory.” (p.352)                                                                                                                                                                                                                                           |
| Stewart and Liou (2017)            | Log total border length and the total number of that states neighbors      | Foreign territorial control                             | Civilian casualties                  | Theory (Geography)                          | “[T]he longer a states borders or the greater its number of neighbors, the more accessible border regions in neighboring states will be to rebels, independent of the dynamics of their conflict with the government. Further, total border length or the number of bordering states is not likely to affect rebel targeting of civilians other than through their effects on the likelihood of rebel groups controlling foreign territory.” (p. 291) |
| Lerman, Sadin and Trachtman (2017) | Born 1946 or 1947                                                          | Public (p 1) versus only private (p 0) health insurance | Support ACA                          | Rules & policy changes (Change in exposure) | “We can confirm across a host of observable covariates that these two age groups are similar on almost every dimension, with the exception of insurance.” (p. 631)                                                                                                                                                                                                                                                                                    |

|                                              |                                                                                                                                  |                            |                                                              |                                |                                                                                                                                                                                                                                                                                                                                                                                            |
|----------------------------------------------|----------------------------------------------------------------------------------------------------------------------------------|----------------------------|--------------------------------------------------------------|--------------------------------|--------------------------------------------------------------------------------------------------------------------------------------------------------------------------------------------------------------------------------------------------------------------------------------------------------------------------------------------------------------------------------------------|
| Grossman, Pierskalla and Boswell Dean (2017) | The number of distinct landmasses; length of medium and small streams; over-time variation in the number of regional governments | Government fragmentation   | Public goods provision                                       | Theory (Geography / diffusion) | “Territorial structure of neighboring countries will affect the local discourse on institutional reforms and increase the likelihood that a country will adopt similar reforms” and “The other two instruments build on the fact that administrative and political boundaries are drawn around geographic landmarks.” (p. 831)                                                             |
| Cirone and Van Coppenolle (2018)             | Random assignment of budget incumbents to bureaux                                                                                | Budget committee service   | Legislator sponsorship on a budget bill                      | Theory (Other)                 | “Conceptually, the competitiveness of the randomly assigned group acts similarly to a form of encouragement design.” (p. 953)                                                                                                                                                                                                                                                              |
| Bhavnani and Lee (2018)                      | Early-career job assignment to districts                                                                                         | Bureaucrats embeddedness   | Proportion of villages with high schools                     | Theory (Other)                 | “[T]he IAS posting orders that we obtained suggest that heuristics such alphabetical order and serial number which are arbitrary and orthogonal to district and officer characteristics are used to match officers to districts.” (p. 78)                                                                                                                                                  |
| Pianzola et al. (2019)                       | Random assignment of the e-mail treatment                                                                                        | Smartvote use              | Vote intention                                               | Experiment                     | NA                                                                                                                                                                                                                                                                                                                                                                                         |
| Arias and Stasavage (2019)                   | Trade shock $\times$ UK bond yield                                                                                               | Government expenditures    | Regular leader turnover                                      | Econometrics (Interaction)     | “The logic here is that when costs of external borrowing are high, a government experiencing a trade shock is more likely to cut expenditures because the option of borrowing to maintain or increase expenditures is too costly. This interaction term is the excluded instrument while the Trade Shock variable is included in both the first- and the second-stage estimates” (p. 1519) |
| Ziaja (2020)                                 | Constructed instrument                                                                                                           | Number of democracy donors | Democracy scores                                             | Econometrics (Interaction)     | “[T]here is no reason to believe that the gender composition of a donor country's parliament should affect democracy in a recipient country directly.” (p.439)                                                                                                                                                                                                                             |
| Schubiger (2021)                             | counterinsurgent mobilization                                                                                                    | exposure to state violence | Location of a community inside or outside the emergency zone | Theory (Geography)             | “Destination choices were typically driven by economic and social factors (e.g., Degregori 1998, 151; Del Pino 1996, 164). Moreover, it is unlikely that local residents were able to anticipate the boundaries of the emergency zones and whether, when, and where they would change over time.” (p.1389)                                                                                 |

|                                      |                                                                      |                                                                               |                     |                                   |                                                                                                                                                                                                                                                       |
|--------------------------------------|----------------------------------------------------------------------|-------------------------------------------------------------------------------|---------------------|-----------------------------------|-------------------------------------------------------------------------------------------------------------------------------------------------------------------------------------------------------------------------------------------------------|
| DiGiuseppe and<br>Shea (2022)        | Echelon corridor                                                     | US support                                                                    | Fiscal<br>capacity  | The-<br>ory(Geography)            | “Like Aklin and Kern (2019), we find that the echelon is plausibly exogenous to a states capacity, property rights, or risk of conflict. Instead, whether a state is located in the echelon corridor is a function of happenstance geography.”(p.777) |
| Lei and Zhou (2022)                  | Whether the city has more than 3 million residents                   | Subway approval                                                               | Mayor promotion     | Rules & policy changes (Fuzzy RD) | “the citys population exceeds 3 million people, and (4) more than 30,000 people per hour are expected to use a subway line”(p.463)                                                                                                                    |
| Urpelainen and Zhang (2022)          | Time trend multiplied by the wind resource of the electoral district | Wind turbine capacity                                                         | Democratic vote     | Economet-<br>rics(Interaction)    | “Validity of the average wind resource instrument hinges on two criteria: relevance and exclusion restriction...”(pp.1313-1314)                                                                                                                       |
| Webster, Connors and Sinclair (2022) | Treatment assignment                                                 | Percentage of angry words that a respondent wrote in emotional recall prompts | Social polarization | Experiment                        | NA                                                                                                                                                                                                                                                    |

**Note:** Justifications are omitted in the case of randomized controlled trials.

## References

- Acharya, Avidit, Matthew Blackwell and Maya Sen. 2016. “The Political Legacy of American Slavery.” *The Journal of Politics* 78(3):621–641.
- Alt, James E, John Marshall and David D Lassen. 2016. “Credible Sources and Sophisticated Voters: When does New Information Induce Economic Voting?” *The Journal of Politics* 78(2):327–342.
- Andrews, Isaiah, James H. Stock and Liyang Sun. 2019. “Weak Instruments in Instrumental Variables Regression: Theory and Practice.” *Annual Review of Economics* 11(1):727–753.
- Arias, Eric and David Stasavage. 2019. “How Large are the Political Costs of Fiscal Austerity?” *The Journal of Politics* 81(4):1517–1522.
- Baccini, Leonardo and Stephen Weymouth. 2021. “Gone for Good: Deindustrialization, White Voter Backlash, and US Presidential Voting.” *American Political Science Review* 115(2):550–567.
- Barth, Erling, Henning Finseraas and Karl O. Moene. 2015. “Political Reinforcement: How Rising Inequality Curbs Manifested Welfare Generosity.” *American Journal of Political Science* 59(3):565–577.
- Bhavnani, Rikhil R. and Alexander Lee. 2018. “Local Embeddedness and Bureaucratic Performance: Evidence from India.” *The Journal of Politics* 80(1):71–87.
- Blair, Robert A, Jessica Di Salvatore and Hannah M Smidt. 2022. “When do UN Peacekeeping Operations Implement their Mandates?” *American Journal of Political Science* 66(3):664–680.
- Blattman, Christopher, Alexandra C. Hartman and Robert A. Blair. 2014. “How to Promote Order and Property Rights under Weak Rule of Law? An Experiment in Changing Dispute Resolution Behavior through Community Education.” *American Political Science Review* 108(1):100–120.
- Bound, John and David A Jaeger. 2000. “Do Compulsory School Attendance Laws Alone Explain the Association between Quarter of Birth and Earnings?” *Research in Labor Economics* 19(4):83–108.
- Carnegie, Allison and Nikolay Marinov. 2017. “Foreign Aid, Human Rights, and Democracy Promotion: Evidence from a Natural Experiment.” *American Journal of Political Science* 61(3):671–683.
- Charron, Nicholas, Carl Dahlström, Mihaly Fazekas and Victor Lapuente. 2017. “Careers, Connections, and Corruption Risks: Investigating the Impact of Bureaucratic Meritocracy on Public Procurement Processes.” *The Journal of Politics* 79(1):89–104.

- Charron, Nicholas and Victor Lapuente. 2013. "Why do Some Regions in Europe Have a Higher Quality of Government?" *The Journal of Politics* 75(3):567–582.
- Chong, Alberto, Gianmarco León-Ciliotta, Vivian Roza, Martín Valdivia and Gabriela Vega. 2019. "Urbanization Patterns, Information Diffusion, and Female Voting in Rural Paraguay." *American Journal of Political Science* 63(2):323–341.
- Cirone, Alexandra and Brenda Van Coppenolle. 2018. "Cabinets, Committees, and Careers: The Causal Effect of Committee Service." *The Journal of Politics* 80(3):948–963.
- Clarke, Damian. 2014. "PLAUSEXOG: Stata Module to Implement Conley et al's Plausibly Exogenous Bounds." <https://econpapers.repec.org/RePEc:boc:bocode:s457832> (accessed July, 2023).
- Colantone, Italo and Piero Stanig. 2018a. "Global Competition and Brexit." *American Political Science Review* 112(2):201–218.
- Colantone, Italo and Piero Stanig. 2018b. "The Trade Origins of Economic Nationalism: Import Competition and Voting Behavior in Western Europe." *American Journal of Political Science* 62(4):936–953.
- Conley, Timothy G, Christian B Hansen and Peter E Rossi. 2012. "Plausibly Exogenous." *The Review of Economics and Statistics* 94(1):260–272.
- Coppock, Alexander and Donald P. Green. 2016. "Is Voting Habit Forming? New Evidence from Experiments and Regression Discontinuities." *American Journal of Political Science* 60(4):1044–1062.
- Croke, Kevin, Guy Grossman, Horacio A. Larreguy and John Marshall. 2016. "Deliberate Disengagement: How Education can Decrease Political Participation in Electoral Authoritarian Regimes." *American Political Science Review* 110(3):579–600.
- De La O, Ana L. 2013. "Do Conditional Cash Transfers Affect Electoral Behavior? Evidence from a Randomized Experiment in Mexico." *American Journal of Political Science* 57(1):1–14.
- Dietrich, Simone and Joseph Wright. 2015. "Foreign Aid Allocation Tactics and Democratic Change in Africa." *The Journal of Politics* 77(1):216–234.
- DiGiuseppe, Matthew and Patrick E Shea. 2022. "Us Patronage, State Capacity, and Civil Conflict." *The Journal of Politics* 84(2):767–782.
- Dower, Paul Castaneda, Evgeny Finkel, Scott Gehlbach and Steven Nafziger. 2018. "Collective Action and Representation in Autocracies: Evidence from Russia's Great Reforms." *American Political Science Review* 112(1):125–147.

- Dube, Oeindrila and Suresh Naidu. 2015. "Bases, Bullets, and Ballots: The Effect of US Military Aid on Political Conflict in Colombia." *The Journal of Politics* 77(1):249–267.
- Eggers, Andrew C, Guadalupe Tuñón and Allan Dafoe. 2021. "Placebo Tests for Causal Inference." *Unpublished manuscript*. [https://pelg.ucsd.edu/Eggers\\_2021.pdf](https://pelg.ucsd.edu/Eggers_2021.pdf).
- Feigenbaum, James J. and Andrew B. Hall. 2015. "How Legislators Respond to Localized Economic Shocks: Evidence from Chinese Import Competition." *The Journal of Politics* 77(4):1012–1030.
- Flores-Macias, Gustavo A. and Sarah E. Kreps. 2013. "The foreign policy consequences of trade: China's commercial relations with Africa and Latin America, 1992–2006." *The Journal of Politics* 75(2):357–371.
- Gehlbach, Scott and Philip Keefer. 2012. "Private Investment and the Institutionalization of Collective Action in Autocracies: Ruling Parties and Legislatures." *The Journal of Politics* 74(2):621–635.
- Gerber, Alan S., Gregory A. Huber and Ebonya Washington. 2010. "Party Affiliation, Partisanship, and Political Beliefs: A Field Experiment." *American Political Science Review* 104(4):720–744.
- Goldstein, Rebecca and Hye Young You. 2017. "Cities as Lobbyists." *American Journal of Political Science* 61(4):864–876.
- Grossman, Guy, Jan H. Pierskalla and Emma Boswell Dean. 2017. "Government Fragmentation and Public Goods Provision." *The Journal of Politics* 79(3):823–840.
- Guiso, Luigi, Paola Sapienza and Luigi Zingales. 2016. "Long-term Persistence." *Journal of the European Economic Association* 14(6):1401–1436.
- Hager, Anselm and Hanno Hilbig. 2019. "Do Inheritance Customs Affect Political and Social Inequality?" *American Journal of Political Science* 63(4):758–773.
- Hager, Anselm and Krzysztof Krakowski. 2022. "Does State Repression Spark Protests? Evidence from Secret Police Surveillance in Communist Poland." *American Political Science Review* 116(2):564–579.
- Hager, Anselm, Krzysztof Krakowski and Max Schaub. 2019. "Ethnic Riots and Prosocial Behavior: Evidence from Kyrgyzstan." *American Political Science Review* 113(4):1029–1044.
- Healy, Andrew and Neil Malhotra. 2013. "Childhood Socialization and Political Attitudes: Evidence from a Natural experiment." *The Journal of Politics* 75(4):1023–1037.
- Henderson, John and John Brooks. 2016. "Mediating the Electoral Connection: The Information Effects of Voter Signals on Legislative Behavior." *The Journal of Politics* 78(3):653–669.

- Hong, Ji Yeon, Sunkyoung Park and Hyunjoo Yang. 2022. "In Strongman We Trust: The Political Legacy of the New Village Movement in South Korea." *American Journal of Political Science* .
- Johns, Leslie and Krzysztof J. Pelc. 2016. "Fear of Crowds in World Trade Organization Disputes: Why Don't More Countries Participate?" *The Journal of Politics* 78(1):88–104.
- Kang, Hyunseung, Yang Jiang, Qingyuan Zhao and Dylan S Small. 2021. "Ivmodel: An R Package for Inference and Sensitivity Analysis of Instrumental Variables Models with One Endogenous Variable." *Observational Studies* 7(2):1–24.
- Kapoor, Sacha and Arvind Magesan. 2018. "Independent Candidates and Political Representation in India." *American Political Science Review* 112(3):678–697.
- Kim, Jeong Hyun. 2019. "Direct Democracy and Women's Political Engagement." *American Journal of Political Science* 63(3):594–610.
- Kocher, Matthew Adam, Thomas B. Pepinsky and Stathis N. Kalyvas. 2011. "Aerial Bombing and Counterinsurgency in the Vietnam War." *American Journal of Political Science* 55(2):201–218.
- Kriner, Douglas L. and Eric Schickler. 2014. "Investigating the President: Committee Probes and Presidential Approval, 1953–2006." *The Journal of Politics* 76(2):521–534.
- Kuipers, Nicholas and Alexander Sahn. 2022. "The Representational Consequences of Municipal Civil Service Reform." *American Political Science Review* pp. 1–17.
- Laitin, David D. and Rajesh Ramachandran. 2016. "Language Policy and Human Development." *American Political Science Review* 110(3):457–480.
- Lei, Zhenhuan and Junlong Aaron Zhou. 2022. "Private Returns to Public Investment: Political Career Incentives and Infrastructure Investment in China." *The Journal of Politics* 84(1):455–469.
- Lelkes, Yphtach, Gaurav Sood and Shanto Iyengar. 2017. "The Hostile Audience: The Effect of Access to Broadband Internet on Partisan Affect." *American Journal of Political Science* 61(1):5–20.
- Lerman, Amy E., Meredith L. Sadin and Samuel Trachtman. 2017. "Policy Uptake as Political Behavior: Evidence from the Affordable Care Act." *American Political Science Review* 111(4):755.
- López-Moctezuma, Gabriel, Leonard Wantchekon, Daniel Rubenson, Thomas Fujiwara and Cecilia Pe Lero. 2022. "Policy Deliberation and Voter Persuasion: Experimental Evidence from an Election in the Philippines." *American Journal of Political Science* 66(1):59–74.

- Lorentzen, Peter, Pierre Landry and John Yasuda. 2014. "Undermining Authoritarian Innovation: The Power of China's Industrial Giants." *The Journal of Politics* 76(1):182–194.
- McClendon, Gwyneth H. 2014. "Social Esteem and Participation in Contentious Politics: A Field Experiment at an LGBT Pride Rally." *American Journal of Political Science* 58(2):279–290.
- Meredith, Marc. 2013. "Exploiting Friends-and-neighbors to Estimate Coattail Effects." *American Political Science Review* 107(4):742–765.
- Nellis, Gareth and Niloufer Siddiqui. 2018. "Secular Party Rule and Religious Violence in Pakistan." *American Political Science Review* 112(1):49.
- Nunn, Nathan. 2008. "The Long-term Effects of Africa's Slave Trades." *The Quarterly Journal of Economics* 123(1):139–176.
- Nunn, Nathan and Leonard Wantchekon. 2011. "The Slave Trade and the Origins of Mistrust in Africa." *American Economic Review* 101(7):3221–3252.
- Olea, José Luis Montiel and Carolin Pflueger. 2013. "A Robust Test for Weak Instruments." *Journal of Business & Economic Statistics* 31(3):358–369.
- Pianzola, Joëlle, Alexander H. Trechsel, Kristjan Vassil, Guido Schwerdt and R. Michael Alvarez. 2019. "The Impact of Personalized Information on Vote Intention: Evidence from a Randomized Field Experiment." *The Journal of Politics* 81(3):833–847.
- Putnam, Robert D, Robert Leonardi and Raffaella Y Nanetti. 1993. *Making Democracy Work: Civic Traditions in Modern Italy*. Princeton, NJ: Princeton University Press.
- Ritter, Emily Hencken and Courtenay R. Conrad. 2016. "Preventing and Responding to Dissent: The Observational Challenges of Explaining Strategic Repression." *American Political Science Review* 110(1):85–99.
- Rueda, Miguel R. 2017. "Small Aggregates, Big Manipulation: Vote Buying Enforcement and Collective Monitoring." *American Journal of Political Science* 61(1):163–177.
- Schleiter, Petra and Margit Tavits. 2016. "The Electoral Benefits of Opportunistic Election Timing." *The Journal of Politics* 78(3):836–850.
- Schubiger, Livia Isabella. 2021. "State Violence and Wartime Civilian Agency: Evidence from Peru." *The Journal of Politics* 83(4):1383–1398.
- Sexton, Renard, Rachel L. Wellhausen and Michael G. Findley. 2019. "How Government Reactions to Violence Worsen Social Welfare: Evidence from Peru." *American Journal of Political Science* 63(2):353–367.
- Spenkuch, Jörg L. and Philipp Tillmann. 2018. "Elite Influence? Religion and the Electoral Success of the Nazis." *American Journal of Political Science* 62(1):19–36.

- Stewart, Megan A. and Yu-Ming Liou. 2017. "Do Good Borders Make Good Rebels? Territorial Control and Civilian Casualties." *The Journal of Politics* 79(1):284–301.
- Stokes, Leah C. 2016. "Electoral Backlash against Climate Policy: A Natural Experiment on Retrospective Voting and Local Resistance to Public Policy." *American Journal of Political Science* 60(4):958–974.
- Tajima, Yuhki. 2013. "The Institutional Basis of Intercommunal Order: Evidence from Indonesia's Democratic Transition." *American Journal of Political Science* 57(1):104–119.
- Trounstein, Jessica. 2016. "Segregation and Inequality in Public Goods." *American Journal of Political Science* 60(3):709–725.
- Urpelainen, Johannes and Alice Tianbo Zhang. 2022. "Electoral Backlash or Positive Reinforcement? Wind Power and Congressional Elections in the United States." *The Journal of Politics* 84(3):1306–1321.
- Van Kippersluis, Hans and Cornelius A Rietveld. 2018. "Beyond Plausibly Exogenous." *The Econometrics Journal* 21(3):316–331.
- Vernby, Kare. 2013. "Inclusion and Public Policy: Evidence from Sweden's Introduction of Noncitizen Suffrage." *American Journal of Political Science* 57(1):15–29.
- Webster, Steven W, Elizabeth C Connors and Betsy Sinclair. 2022. "The Social Consequences of Political Anger." *The Journal of Politics* 84(3):1292–1305.
- West, Emily A. 2017. "Descriptive Representation and Political Efficacy: Evidence from Obama and Clinton." *The Journal of Politics* 79(1):351–355.
- Wood, Abby K and Christian R Grose. 2022. "Campaign Finance Transparency Affects Legislators Election Outcomes and Behavior." *American Journal of Political Science* 66(2):516–534.
- Zhu, Boliang. 2017. "MNCs, Rents, and Corruption: Evidence from China." *American Journal of Political Science* 61(1):84–99.
- Ziaja, Sebastian. 2020. "More Donors, more Democracy." *The Journal of Politics* 82(2):433–447.
